# Supplementary material for: Optimal Stateless Model Checking of Transactional Programs under Causal Consistency
Source: arXiv:2211.09020 source file (2023-01-16)
Supplement: Supplementary file 1 [file appendix.tex]

\centerline{\Large{Appendix}}

%\counterwithin{theorem}{section}
%\counterwithin{lemma}{section}

The appendix contains the following sections.
\begin{enumerate}
\item Programs under $\ccvt$ 
\begin{enumerate}
	\item The proof of Theorem \ref{thm-legal} (Appendix \ref{app:legal})
	\item The proof of Theorem \ref{ccv-sat} (Appendix \ref{app:ccv-sat})
	\item Properties of the fulfilled semantics where we show that all 
	generated traces are fulfilled and $\models \ccvt$. This proves Lemma \ref{lem:satcons} (Appendix \ref{app:satcons})
		\item The proof of Lemma \ref{lemma:poly} (Appendix \ref{app:poly})
	\item A new incremental semantics that is equivalent to the total semantics  
	(Appendix \ref{app:inc}). The incremental semantics defines the total traces in a step by step fashion, and simplifies the proof of Theorem \ref{thm:ccv}.
		\item The proof of Theorem \ref{thm:ccv} (Appendix \ref{app:thm:ccv})
	\item Proof of the completeness of the DPOR algorithm (Appendix \ref{app:complete-ccv}).
%	\item The DPOR algorithm on an example (Appendix \ref{app:dpor-eg})
\end{enumerate}
\item Programs under $\critw$
\begin{itemize}
\item[(a)] 	Operational Semantics of $\cc$ from \cite{lmcs:7149} (Appendix \ref{app:cc})
\item[(b)] Axiomatic Semantics for $\cc$ (Appendix \ref{app:ccsum})
\item[(c)] Equivalence of $\cc$ axiomatic semantics with the operational semantics (Theorem \ref{thm:cc-legal}, Appendix \ref{app:ccsum})
\item[(d)] $\cc$ Fulfilled Semantics (Appendix \ref{app:ccful})
\item[(e)] DPOR for $\cc$, soundness, completeness and optimality (Appendix \ref{app:cc-dpor})
\end{itemize}

%\item Programs under $\critm$
%\begin{itemize}
%\item[(a)]Operational Semantics for $\cm$	from \cite{lmcs:7149} (Appendix \ref{app:cm})
%\item[(b)]Successor computation in $\cm$ execution summaries is NP-c(Appendix \ref{app:npc}) 
  
%\end{itemize}
\item Experimental Evaluation
\begin{itemize}
	\item [(a)] The litmus test where the assertion violating execution is not in $\ccvt$, for any grouping of instructions as transactions (Appendix \ref{app:lit})
	\item[(b)]Uncited programs used in Table \ref{tab:class} (Appendix \ref{app:tab3-p})
	\item[(c)]  Time taken by $\ccvt, \cc$ for all 3 versions of the benchmarks 
 	  used in Table \ref{tab:class} (Appendix \ref{app:tab3})
	  
\end{itemize}

\end{enumerate}

\newpage
\begin{center}
\Large{\bf{Causal Convergence $\ccvt$ }}
	
\end{center}
\section{Equivalence of the Axiomatic and Operational Semantics for $\ccvt$}

\subsection{Proof of Theorem \ref{thm-legal}}
\label{app:legal}
\begin{proof}
First let us go from traces to legal execution summaries. 
\subsection*{$\ccvt$-consistent Traces to Legal Execution Summaries}

Consider a partial trace $\tau=(\tran, \textcolor{red}{po},\textcolor{blue}{rf},-)$. Assume that we can extend it to a total, $\ccvt$ consistent trace $\tau'=(\tran, \textcolor{red}{po},\textcolor{blue}{rf},\textcolor{orange}{co})$. Given $\tau'$, we show that 
we can construct a $\tau'$-consistent, legal execution summary.

%Consider the trace $\tau$ corresponding to an execution $E$.  Assume that we can extend it to a $\ccvt{}$ consistent trace $\tau ^\prime =\langle E_t,\textcolor{red}{po},\textcolor{blue}{rf},\textcolor{orange}{co} \rangle$. Then we know that [$\textcolor{red}{po} \cup \textcolor{blue}{rf}\cup \textcolor{orange}{co} \cup \textcolor{violet}{fr}^x$] is acyclic. Moreover, for each variable $x$, the transactions in $E_t^{w,x}$ are totally ordered. 

Assume that we have processes $p_1, p_2, ... p_n$ 
in the concurrent program $\mathcal{P}$ over the set of transactions $\tran$.  Define for each $i$, 
\begin{itemize}
	\item  Let $A_i$ be the set of all transactions $t \in \tran$ issued in process $p_i$, 
%	
%	to events $\issueact(p_i,t)$, over all processes $p_i$ and transactions $t_i \in \tran$. 
%%	
%	
%	appears in the execution summary of $E\}$ be all transactions $t$ for which 
%	$\issueact(p_i,t)$ appears in the execution summary of $E$
	 	\item Let $A^\prime_i = A_i \cup \tran^w$. $A'_i$ 
	 	contains all transactions issued in process $p_i$, as well as all transactions 
	 		 	in $\tran$ having a write instruction,
	 	 	\item Define the relation $<_i = ((hb \cap (A^\prime_i \times A^\prime_i)) \cup ((A_i \times (A^\prime_i \setminus A_i)) \setminus hb^{-1}) $
where $hb= (\textcolor{red}{po} \cup \textcolor{blue}{rf})^+$. Relation $<_i$ is a strict partial order.
\smallskip 

$hb \cap (A^\prime_i \times A^\prime_i)$ is built on pairs of transactions $(t,t')$ where $t,t'$ are issued in $p_i$, representing $\tpo$, as well as pairs $(t,t')$ 
such that $t$ is delivered to $p_i$ and $t'$ is issued in $p_i$ after that, representing a $\trf$. Likewise, 
$((A_i \times (A^\prime_i \setminus A_i))\setminus hb^{-1}))$ is built on pairs  (i) $(t, t')$ where $t$ is issued in $p_i$ and $t'$ is delivered to $p_i$ but not issued in $p_i$, such that  
$(t', t) \notin hb$.

%(\issueact(p_i,t), \storeact(p_j,t'))$ 
% such that 
%$(t', t) \notin hb$, with $t'$ not issued in $p_i$, or (ii) 
% $(\storeact(p_i,t), \storeact(p_j,t'))$ 
% such that 
%$(t', t) \notin hb$, with $t$ issued in $p_i$ and $t'$ not issued in $p_i$. 
%Note that $p_j$ can be $p_i$.  

%If we think in terms of execution summaries, then $hb \cap (A^\prime_i \times A^\prime_i)$ is built on pairs $(\issueact(p_i,t), \issueact(p_i,t'))$ (represents $\textcolor{red}{po}$) as well as $(\storeact(p_i,t), \issueact(p_i, t'))$ (represents $\textcolor{blue}{rf}$).
%Likewise,  $((A_i \times (A^\prime_i \setminus A_i))\setminus hb^{-1}))$ is built on 
%pairs (i) $(\issueact(p_i,t), \storeact(p_j,t'))$ 
% such that 
%$(t', t) \notin hb$, with $t'$ not issued in $p_i$, or (ii) 
% $(\storeact(p_i,t), \storeact(p_j,t'))$ 
% such that 
%$(t', t) \notin hb$, with $t$ issued in $p_i$ and $t'$ not issued in $p_i$. 
%Note that $p_j$ can be $p_i$.  

\end{itemize}
Now define two sets of events $T, T'$ as follows.
\begin{itemize}
	\item Let $T = \{\issueact(p_i,t) \mid 1 {\le} i {\le} n, t \in A_i\} \cup \{ \storeact(p_i,t) \mid 1 {\le} i {\le} n, t \in A^\prime_i\setminus A_i\}$. 
	%$\setminus A_i)\}$.  
	Thus, $T$ consists of all transactions $t$ issued in process $p_i$, or those transactions $t$  delivered to process $p_i$ (but not issued 
	in $p_i$). 
	\item Let $T' = \{\issueact(p_i,t) \mid 1 \le i \le n, t \in A_i \cap \tran^w\}$. $T'$ consists of all transactions issued in process $p_i$ 
	which also have a write instruction.  
\end{itemize}
We define the following relations on $T,T'$:

\begin{itemize}
\item [1.] $B_1 = \{ \langle x(p_i,t), y(p_i, t^\prime) \rangle \in T \times T  \mid x, y \in \{\issueact, \storeact\} \text{ and } t <_i t^\prime \}$.
%, and $x, y \in \{\issueact, \storeact\}$.
      $B_1$ relates issue and delivery events in the {\bf{same}} process $p_i$. 
    $B_1$ has pairs $(\issueact(p_i,t), \issueact(p_i,t'))$ as well as 
    $(\storeact(p_i,t), \issueact(p_i,t'))$ covering 
      $\textcolor{red}{po} \cup \textcolor{blue}{rf}$ relations in each $p_i$.
In addition, $B_1$ also has the pairs $(\storeact(p_i,t), \storeact(p_i,t'))$ 
as well as $(\issueact(p_i,t), \storeact(p_i,t'))$.  
%      In addition, $B_1$ also has pairs $(\issueact(p_i,t), \storeact(p_i,t'))$ 
      By definition of 
    $\textcolor{red}{po} \cup \textcolor{blue}{rf}$ and $<_i$, $B_1$ is irreflexive (or acyclic).
     \item [2.] $B_2 = \{ \langle \issueact(p_i,t), \storeact(p_j, t) \rangle  \in T' \times T \}$.  
%    \{(\storeact(p_i,t), \storeact(p_j,t) \in T \times T  \mid t$ is issued in $p_i\}$. 
%     
      $B_2$ relates the issue $\issueact(p_i,t)$ of each transaction $t$ in process $p_i$ to its corresponding delivery $\storeact(p_j,t)$ in some process $p_j$. 
%      and also orders self delivery of transactions  
%      before delivering to other processes. 
       Clearly, $B_2$ is also irreflexive.  
    \item[3.] $B_3 = \{ \langle \issueact(p_i,t), \issueact(p_j, t^\prime) \rangle  \in T' \times T' \mid t [\textcolor{orange}{co}] t'\}$.
     $B_3$ models the  $[\textcolor{orange}{co}]$ relation, and is a total  irreflexive order.
 \end{itemize}
Indeed $B_1 \cup B_2 \cup B_3$ is irreflexive. We build an execution summary using $(B_1 \cup B_2 \cup B_3)$, and the relation $<$ induced by $B_1, B_2, B_3$. The events in the execution summary are obviously, $Ev=\{\issueact(p,t), \storeact(p,t') \mid$ $t, t' \in \tran$ and  $p \in \mathbb{P}\}$, and the ordering $<$ is defined as 
$(a,b) \in (B_1 \cup B_2 \cup B_3)^+ \Rightarrow a < b$. 

\subsubsection{$<$ is a total order}: 
To show that $(Ev,<)$ is a legal execution summary, one of the things to show is that $<$ is a total order on the events $Ev$. To this end, we show that 
$(B_1 \cup B_2 \cup B_3)^+$ is irreflexive.

\begin{lemma}
	If $\langle x(p_i,t_1) , \issueact(p_j,t_2) \rangle \in (B_1 \cup B_2)^+$ then $t_1 [\tpo \cup \trf]^+ t_2$.
	\label{lem:porf}
\end{lemma}
\begin{proof}

 We prove this using induction. 
 If $(x(p_i,t_1) , \issueact(p_j,t_2)) \in (B_1 \cup B_2)^+$, 
 then there is a sequence $x_1(p_{i_1},t_{j_1}) < x_2(p_{i_2},t_{j_2}) <  \cdot \cdot \cdot x_{n-1}(p_{i_{n-1}},t_{j_{n-1}}) < x_n(p_{i_n},t_{j_n})$, where $x_1(p_{i_1},t_{j_1}) = x(p_i,t_1)$ and $x_n(p_{i_n},t_{j_n}) =\issueact(p_j,t_2)$. 
\smallskip

\noindent{\bf{Base Cases}}. The base cases are $(i)$ $\langle x(p_1,t_1), \issueact(p_2,t_2) \rangle \in B_1$, this case is trivial. $(ii)$ $\langle x_1(p_1,t_1), x_2(p_2,t_2) \rangle \in (B_1 \cup B_2)$ and  $\langle x_2(p_2,t_2), \issueact(p_3,t_3) \rangle \in (B_1 \cup B_2)$. For $(ii)$ we consider the following:
\begin{itemize}
\item[(1)] $ \langle x_1(p_1,t_1), x_2(p_2,t_2) \rangle \in B_1$ and $ \langle x_2(p_2,t_2), \issueact(p_3,t_3) \rangle \in B_1$. It follows that $p_1 = p_2 = p_3$. Hence we have $t_1[\tpo \cup \trf]^+ t_3$.

\item[(2)]  $ \langle x_1(p_1,t_1), x_2(p_2,t_2) \rangle \in B_2$ and $ \langle x_2(p_2,t_2), \issueact(p_3,t_3) \rangle \in B_1$.  \\ 
$\langle x_1(p_1,t_1), x_2(p_2,t_2) \rangle \in B_2$ implies that $t_1 = t_2$ and $x_2$ is $\storeact$ event. Since $\langle x_2(p_2,t_2),  \issueact(p_3,t_3) \rangle \in B_1$ we have $p_2 = p_3$ and $t_2[\tpo \cup \trf]^+ t_3$. Hence we have $t_1[\tpo \cup \trf]^+ t_3$.
\end{itemize}

\noindent{\bf{Inductive Step}}. Assume the result for all sequences 
 of length $\leq n-2$, that is, whenever there is a sequence $x_1(p_{i_1},t_{j_1}) < x_2(p_{i_2},t_{j_2}) <  \cdots  <x_{n-2}(p_{i_{n-2}},t_{j_{n-2}})$ with  $x_{n-2}(p_{i_{n-2}},t_{j_{n-2}})=\issueact(p_{i_{n-2}},t_{j_{n-2}})$, we have $t_{j_1} [\tpo \cup \trf]^+ t_{j_{n-2}}$.

 Consider a sequence of length $n$. 
Let $\langle x_{n-2}(p_{i_{n-2}},t_{j_{n-2}}), 
x_{n-1}(p_{i_{n-1}},t_{j_{n-1}}) \rangle \in (B_1 \cup B_2)$ \\ and $ \langle x_{n-1}(p_{i_{n-1}},t_{j_{n-1}}), x_n(p_{i_n},t_{j_n}) \rangle \in (B_1 \cup B_2)$, where $x_n(p_{i_n},t_{j_n}) =\issueact(p_j,t_2)$. Here again we have two cases:
\begin{itemize}
\item[(1)] $\langle x_{n-2}(p_{i_{n-2}},t_{j_{n-2}}), x_{n-1}(p_{i_{n-1}},t_{j_{n-1}}) \rangle, \langle x_{n-1}(p_{i_{n-1}},t_{j_{n-1}}), x_n(p_{i_n},t_{j_n}) \rangle \in B_1$. It follows that $p_{i_{n-2}} = p_{i_{n-1}} = p_{i_{n}} = p_j$. Hence we have $t_{j_{n-2}} [\tpo \cup \trf]^+ t_{j_n}$. From the inductive hypothesis we have $t_1 [\tpo \cup \trf]^+ t_{j_{n-2}}$. Hence we have $t_1 [\tpo \cup \trf]^+ t_{j_n}$, i.e. $t_1 [\tpo \cup \trf]^+ t_2$. 

\item[(2)] Consider the case when $\langle x_{n-2}(p_{i_{n-2}},t_{j_{n-2}}), x_{n-1}(p_{i_{n-1}},t_{j_{n-1}}) \rangle \in B_2$, and \\ $ \langle x_{n-1}(p_{i_{n-1}},t_{j_{n-1}}), x_n(p_{i_n},t_{j_n}) \rangle \in B_1$.

 Since $\langle x_{n-2}(p_{i_{n-2}},t_{j_{n-2}}), x_{n-1}(p_{i_{n-1}},t_{j_{n-1}}) \rangle \in B_2$, it follows that $x_{n-1}$ is a $\storeact$ event and $ t_{j_{n-2}} = t_{j_{n-1}}$. Since $ \langle x_{n-1}(p_{i_{n-1}},t_{j_{n-1}}), x_n(p_{i_n},t_{j_n}) \rangle \in B_1$, we have $p_{i_{n-1}} = p_{i_n} = p_j$ and $t_{j_{n-1}} [\tpo \cup \trf]^+ t_{j_n}$, i.e $t_{j_{n-2}} [\tpo \cup \trf]^+ t_2$. From the inductive hypothesis we have $t_1 [\tpo \cup \trf]^+ t_{j_{n-2}}$. Hence we have $t_1 [\tpo \cup \trf]^+ t_{j_n}$, i.e. $t_1 [\tpo \cup \trf]^+ t_2$.
\end{itemize}

\end{proof}

\begin{lemma}
$<$ can be extended to a total order	. 
\label{lem:tot}
\end{lemma}
\begin{proof}
We show that $(B_1 \cup B_2 \cup B_3)^+$ is irreflexive. This allows us to extend $<$ to a total order on $Ev$. First of all, notice that $B_1 \cup B_2 \cup B_3$ is irreflexive since each of $B_1, B_2, B_3$ are irreflexive. 
We first show that $(B_1 \cup B_2)^+$ is irreflexive, and then use this to argue the irreflexivity of $(B_1 \cup B_2 \cup B_3)^+$. 

\smallskip

\noindent{\bf{Irreflexivity of  $(B_1 \cup B_2)^+$}}. 
 Assume otherwise. To obtain a $(x,x) \in (B_1 \cup B_2)^+$, we must 
 compose $B_1, B_2$, as individually both $B_1, B_2$ are reflexive. 
  
  \begin{enumerate}
  	\item Consider the case when we have  $\langle x(p_i,t_1),\issueact(p_j,t_2) \rangle, \langle \issueact(p_j,t_2), y(p_k,t_3) \rangle \in B_1 \cup B_2$, and $\langle y(p_k,t_3), x(p_i,t_1) \rangle \in (B_1 \cup B_2)^+$. Since $\langle x(p_i,t_1),\issueact(p_j,t_2) \rangle \in B_1$ and $\langle y(p_k,t_3), x(p_i,t_1) \rangle \in (B_1 \cup B_2)^+$, we have $\langle y(p_k,t_3), \issueact(p_j,t_2) \rangle \in (B_1 \cup B_2)^+$. 
  	
  	By Lemma \ref{lem:porf}, it follows that $t_3 [\tpo \cup \trf]^+t_2$. 
  	\begin{itemize}
  	\item If $y(p_k,t_3) = \issueact(p_k,t_3)$.
 
 Then  $\langle \issueact(p_j,t_2),y(p_k,t_3) \rangle = \langle \issueact(p_j,t_2),\issueact(p_k,t_3) \rangle\in B_1$.  
  	Hence  $p_j = p_k$ and $t_2 [\tpo] t_3$. Thus we get a cycle $t_3 [\tpo \cup \trf]^+t_2 [\tpo] t_3$. This contradicts the fact that $(\tpo \cup \trf)^+$ is irreflexive. 
  	\item If $y(p_k,t_3) = \storeact(p_k,t_3)$.
  	
  	Then $\langle \issueact(p_j,t_2),$ $y(p_k,t_3) \rangle =\langle \issueact(p_j,t_2),\storeact(p_k,t_3) \rangle \in B_2$ and $t_2 = t_3$, i.e we get $t_3 [\tpo \cup \trf]^+t_3$. This contradicts the fact that $(\tpo \cup \trf)^+$ is irreflexive. 
  	
  	\end{itemize}

  		\item Another possibility is $\langle \issueact(p_i,t_1),\storeact(p_j,t_2) \rangle \in B_2$, $\langle \storeact(p_j,t_2),y(p_k,t_3) \rangle \in B_1 \cup B_2$, and $\langle y(p_k,t_3), \issueact(p_i,t_1) \rangle \in (B_1 \cup B_2)^+$.
  		Combining  	$\langle y(p_k,t_3), \issueact(p_i,t_1) \rangle \in (B_1 \cup B_2)^+$ and \\ $\langle \issueact(p_i,t_1),\storeact(p_j,t_2) \rangle \in B_2$, we get 
  		 $\langle y(p_k,t_3),\storeact(p_j,t_2) \rangle \in (B_1 \cup B_2)^+$. 
  		 
  \begin{itemize}
  \item If 	$y(p_k,t_3)=\issueact(p_k,t_3)$.

  Then  $\langle \storeact(p_j,t_2),y(p_k,t_3) \rangle  = 
   \langle \storeact(p_j,t_2),\issueact(p_k,t_3) \rangle  \in B_1$. 
   Then $p_j=p_k$ and $t_2  [\tpo] t_3$. Then we get the cycle 
   $t_3 [\tpo \cup \trf]^+t_2[\tpo] t_3$.

  \item  If 	$y(p_k,t_3)=\storeact(p_k,t_3)$.

  Then $\langle \storeact(p_j,t_2),y(p_k,t_3) \rangle  =
    \langle \storeact(p_j,t_2),\storeact(p_k,t_3) \rangle  \in B_1$.
   Then $p_j=p_k$ and $t_2  [\tpo] t_3$. Then we get the cycle 
   $t_3 [\tpo \cup \trf]^+t_2[\tpo] t_3$. 
    \end{itemize}

  \end{enumerate}
Thus, 	 $(B_1 \cup B_2)^+$ is irreflexive.

\smallskip

\noindent{\bf{ Irreflexivity of $(B_1 \cup B_2 \cup B_3)^+$}}. 
   Assume otherwise. To obtain $(x,x) \in (B_1 \cup B_2 \cup B_3)^+$, we must compose  $(B_1 \cup B_2)^+$ and $B_3$ since, individually, 
   $(B_1 \cup B_2)^+$ and $B_3$ are irreflexive. To this end, consider 
    $\langle x(p_i,t_1) , \issueact(p_j,t_2) \rangle \in (B_1 \cup B_2)^+$ 
    and $\langle \issueact(p_k,t_3) , \issueact(p_l,t_4) \rangle \in B_3$.
         Then we have  $t_1 [\tpo \cup \trf]^+ t_2$ and  $t_3 [\tco] t_4$.
  Assume a cycle in $(B_1 \cup B_2 \cup B_3)^+$ involving $t_1, t_2, t_3, t_4$, 
  of the form
            $t_0 [\tpo \cup \trf]^+ t'_0 [\tco] t_1 [\tpo \cup \trf]^+ t'_1 [\tco] \cdot \cdot \cdot [\tpo \cup \trf]^+ t'_{n-1} [\tco] t_n [\tpo \cup \trf]^+ t'_n$
            where $t_0 = t'_n$. This contradicts the fact that $(\tpo \cup \trf \cup \tco)$ is acyclic.

 The irreflexivity of $(B_1 \cup B_2 \cup B_3)^+$ shows that we can extend $<$ to a total order.

%\qed
\end{proof}
We now show how to build an execution summary  $S=(Ev,<)$ using the events $Ev$, and the total order $<$ which is legal and $\tau'$-consistent. Let the  execution summary be $S=\sigma_0 \xrightarrow[]{\ell_1} \sigma_1 \xrightarrow[]{\ell_2} \sigma_2 \xrightarrow[]{\ell_3} \sigma_3 \cdots \xrightarrow[]{\ell_{n-1}} \sigma_{n-1} \xrightarrow[]{\ell_n} \sigma_n$. 

\noindent{\bf{$S=(Ev,<)$ is $\tau'$-consistent}}. We show that $S$ satisfies all the conditions to be $\tau'$-consistent below. 
\begin{itemize}
	\item[$\star$]  First, each transaction $t \in \tran$ is issued in some unique process $p_i$. This is ensured by the total order $<$.  
\item[$\star$] For $t, t' \in \tran$, if $t[\textcolor{red}{po}] t'$ in $\tau'$, we have $t <_i t'$ by definition. This gives us $(\issueact(p,t), \issueact(p,t')) \in B_1$, giving $\ell_i=\issueact(p,t), \ell_j=\issueact(p,t')$ in $S$ with $i < j$.   
\item[$\star$] For $t, t' \in \tran^w$, if $t[\tco] t'$ in $\tau'$, 
then $(\issueact(p_i,t), \issueact(p_j,t')) \in B_3$. Then we have 
$\ell_i=\issueact(p_i,t), \ell_j=\issueact(p_j,t')$ with $i < j$. 

\item[$\star$] For $t, t' \in \tran$, if $t' [\trf^x] t$, then we have 
$t' <_i t$ by definition of $<_i$.  This gives us $(\storeact(p,t'), \issueact(p,t)) \in B_1$, giving $\ell_i=\storeact(p,t'), \ell_j=\issueact(p,t)$ with $i < j$ in $S$, $t' \in \tran^{w,x}, t \in \tran^{r,x}$.  It remains to argue that 
$t$ reads from the latest transaction which has written on $x$ and delivered to it,  and that is $t'$. We show this below in (1). 

\smallskip 
%
%Assume for a contradiction that  $t'' \in \tran^{w,x}$ such that  $t' [\tco^x] t''$, and 
%$\storeact(p_i,t') < \storeact(p_i, t'') < \issueact(p,t)$. Then by Lemma \ref{lem:porf}, we have $t'' [\tpo \cup \trf]^+ t$,  $t' [\tpo \cup \trf]^+ t$. Coupling  $t' [\trf^x] t$, $t'' [\tpo \cup \trf]^+ t$ along with the fact that $\tau' \models \ccvt$ we obtain $t'' [\tco^x] t'$, which contradicts our assumption. 
%
%
%Thus, we can ensure that 
%$\neg( \exists t'' \in \tran^{w,x}[\storeact(p,t'')=\ell_k, i<k<j \wedge 
%   t' [\tco^x] t''])$. 

\end{itemize}

 \noindent{\bf{   $S=(Ev,<)$ is a legal  execution summary}}. 
	 To show this, we must show the three conditions of legality hold good. 
	
		Recall  the function
	$S.hb : \tran^r \rightarrow \powerset(\tran^w)$ which associates a transaction $t$ having a read event, with the set of  transactions $t'$ it can read from, defined as	
	 $S.hb(t)=\{t' \in \tran^w \mid 
	\storeact(p,t') < \issueact(p,t)\}$.
	 %and $t$ can perform an external read  from $t'\}$.  
	Recall also,  
	the function $S.lw : \tran^r \times \mathcal{V} \rightarrow \tran^w$, 
	which associates to each transaction $t \in \tran^r$, the latest transaction in $[\tco]^x$ order it can read $x \in \mathcal{V}$ from. This is defined 
	as  $S.lw(t,x)=\{t' \mid t' \in S.hb(t) \cap \tran^{w,x}, t \in \tran^{r,x}$ and $\forall t'' \in S.hb(t) \cap \tran^{w,x}, t''.id \leq t'.id\}$
	
%	
%	 there is no $t'' \in S.hb(t) \cap \tran^{w,x}$ such that 
%	$t'[\textcolor{red}{co}]t''$ and  $\storeact(p,t') <   \storeact(p,t'') < \issueact(p,t)\}$. 
%	
	\begin{itemize}
		\item[(1)] The first condition is to show that,  each transaction $t$ in process $p_i$ reads from the latest write, i.e. $(S.lw(t,x) = t')$ when $t' [\trf^x] t$.
		 Let $(\storeact(p_i,t'), \issueact(p_i,t)) \in B_1$ with $t' \in \tran^{w,x}, t \in \tran^{r,x}$, $t' \in S.hb(t)$, and $t'[\trf^x]t$. We show that $S.lw(t,x) = t'$. 
		 
		 \smallskip 
		 
		 Assume otherwise, that is, there exists a transaction $t'' \in \tran^{w,x}$ such that 
$(\storeact(p_i,t''), \issueact(p_i,t)) {\in} B_1$ and $S.lw(t,x) = t''$. By Lemma \ref{lem:porf}, $t'' [\tpo \cup \trf]^+ t$. Since $t' \in S.hb(t)$ and $S.lw(t,x) =t''$, we have $t'.id \leq t''.id$.  Using $t' [\trf^x] t$, 
$t'' [\tpo \cup \trf]^+ t$ and the fact that $\tau' \models \ccvt$, we obtain 
$t'' [\tco^x] t'$. This implies that $t''.id < t'.id$ since 
we can have $\storeact(p,t'')<\issueact(p,t')$ but not the other way around, 
since $t'' [\tco^x] t'$ implies $\issueact(-,t'') < \issueact(-,t')$. 
 This however contradicts $t'.id \leq t''.id$, and therefore contradicts 
 $S.lw(t,x) =t''$. Thus, $S.lw(t,x) =t'$.

		\item[(2)] The second condition to prove is this : For transactions $t,t' \in \tran^w$, if $\storeact(p,t) < \issueact(p,t')$, then $\storeact(p',t) < \storeact(p',t')$ for 
		any $p' \neq p$. 
		If we have $\storeact(p,t) < \issueact(p,t')$, then 
	$(\storeact(p,t), \issueact(p,t')) \in B_1$. By definition of $B_1$, then we have $t<_p t'$.  By Lemma \ref{lem:porf}, we have $(t,t') \in$ [$\tpo \cup \trf$]$^+$. By definition of $<_{p'}=hb \cap A'_{p'} \times A'_{p'}$, we obtain $t <_{p^\prime} t'$ since $t, t' \in \tran^w$.
		 By $B_1$, $t <_{p'} t'$ gives 
		$\storeact(p',t) < \storeact(p',t')$.

		%and $t [\textcolor{red}{po} \cup \textcolor{blue}{rf}]^+ t'$.
%		 For a contradiction, assume that $\storeact(p',t') < \storeact(p',t)$. 
%		 
%		 
%		 
%		 
%		 Then we have $t' <_{p'} t$ by $B_1$ again. The definition of $t' <_{p'} t$ has two possibilities : one which allows 
%		 $t'[hb]t$, and the second one, where $\neg(t' [hb] t)$. 
%		 
%		 
%		 
%%		 $t \in \tran^w$ 
%%		 and $\issueact(p',t')$. 
%%		 
%		  We consider both cases below.
%		 
%\begin{itemize}
%\item  We cannot have $t'[hb]t$ since we already have $\storeact(p,t) < \issueact(p,t')$ which already implies $t [hb] t'$.
%\item Consider the case where we have $\neg(t' [hb] t)$. 
%
%If we have $\issueact(p',t)$, then we also have 
%	$\issueact(p',t) < \storeact(p',t) < \storeact(p',t')$.  
%
%If we have $\issueact(p'',t)$ for $p'' \neq p$, then 
%$\issueact(p'',t) < \storeact(p'',t) < \storeact(p,t) < \issueact(p,t')$ 
%giving $t [co] t'$

%
%By assumption we have $\storeact(p',t') < \storeact(p',t)$. This along with 
%$\storeact(p,t)< \issueact(p,t')$ gives 
%$$\storeact(p,t)< \issueact(p,t')< \storeact(p,t') < \storeact(p',t') < \storeact(p',t)$$

%$t \in \tran^w$ 
%		 and $\issueact(p',t')$. Then we have $\issueact(p',t') < \storeact(p',t') < \storeact(p',t)$. If we have 
%		 $\issueact(p',t') < \issueact(-,t)$, then by $B_3$ we have 
%		 $t'[co]t$. By assumption that $\tau'$ is $\ccvt$ consistent, we then also have $t'[hb]t$.  

%\end{itemize}		 
		 
\item[(3)] The 	third condition is to show this : for each transaction $t$ and processes $p, p'$, $\issueact(p,t) < \storeact(p',t)$. This is given to us by $B_2$ already. 
		 
	\end{itemize}
	 
Thus, we have shown that we can construct a $\tau'$-consistent, legal execution summary from the $\ccvt$ consistent trace $\tau'$.

\subsection*{Legal Execution Summaries to $\ccvt$-consistent Traces}
For the converse direction, assume that we begin with a legal execution summary 
$\exsum(\rho)$ corresponding to an execution $\rho$. First, we define the trace 
corresponding to $\rho$, denoted $\tau=\traceof{\rho}$ following what we did in the main paper. To recall, given $\exsum(\rho)=(\evsum,<)$, 
 \begin{itemize}
     \item For transactions $t, t'$, define $t$ [\textcolor{red}{po}] $t'$ when  we have $ev_1=\issueact(p,t)$ 
     and $ev_2=\issueact(p,t')$  such that $ev_1 < ev_2$ in $\tau$. This corresponds to the order of transactions issued in process $p$.  
          $\tpo$ does not relate the initializer transactions.  
     
     \item $t$ [\textcolor{blue}{rf}] $t'$ relates transactions with delivery and issue events.  
      If there exists $ev_1=\storeact(p,t)$ and $ev_2=\issueact(p,t')$ such that $ev_1 < ev_2$ in $\tau$ such that $t'$ performs an \emph{external read} of some variable $x$ and $ev_1$ is the last event in $\tau$ before $ev_2$ that writes to $x$,   $t=S.lw(t',x)$. 
      We say that $t'$ performs an \emph{external read} on a variable $x$ in the  run $\rho$ if $\rho$ has the read event $r(p,t',x,v)$ which is not preceded by a $w(p,t',x,v)$.
      
      The variable $x$ can be made explicit by defining  $t [\textcolor{blue}{rf}^x] t'$.
     
     \item $t$ [\textcolor{orange}{co}] $t '$ relates transactions 
     writing on common variables. If there are events $ev_1=	\issueact(p,t)$ 
     and $ev_2=\issueact(q,t')$ such that $ev_1 < ev_2$ in $\tau$, 
     such that $t_1, t_2$ both write on $x$, then $t$ [\textcolor{orange}{co}] $t '$.  Note that the transaction 
     $init_x$ is such that $init_x [\textcolor{orange}{co}] t$ for all transitions  $t \in \tran(\rho)^{w,x}$. 
     
      \end{itemize}

We now show that the trace $\tau$ as defined above is $\ccvt$ consistent. For this, we have to show the following. 
\begin{enumerate}
%	\item $\tau$ is total. This is true since we relate all pairs of transactions having writes on common variables.
	\item For each variable $x$, $\textcolor{orange}{co}^x$ respects 
	$[\textcolor{red}{po} \cup \textcolor{blue}{rf}^x]^+$. Assume $t [\textcolor{red}{po} \cup \textcolor{blue}{rf}^x]^+ t'$ for $t,t' \in \tran(\rho)^{w,x}$. 
	Then we have a sequence $\issueact(p,t) < \issueact(p,t^1_p)< \dots  <\issueact(p,t^n_p) 
	<\storeact(p,t^n_p) < \storeact(p',t^n_p) < \issueact(p',t^1_{p'}) < \dots \issueact(q, t')$. This gives  $\issueact(p,t) <  \issueact(q, t')$. 
	By definition,  $t [\textcolor{orange}{co}]^x t'$.
	\item Assume $t_1 [\textcolor{blue}{rf}^x] t_2$ and $t_3 [\textcolor{red}{po} \cup \textcolor{blue}{rf}]^+ t_2$.
	We show that $t_3 [\textcolor{orange}{co}^x] t_1$. 
	\smallskip 
	
	Assume otherwise, that is, $t_1 [\tco] t_3$.
	Since $t_3 [\tpo \cup \trf]^+ t_2$, we have $\storeact(p_i,t_3) < \issueact(p_i,t_2)$, i.e. $t_3 \in S.hb(t_2)$. 
	Since $t_1 [\tco] t_3$, we have $\issueact(p_j,t_1) < \issueact(p_k,t_3)$. 
	Together with	$t_1 , t_3 \in S.hb(t_2)$, we have $t_1 \neq S.lw(t_2,x)$. 
	Since $t_1 [\trf^x] t_2$, we have $t_1 \in S.hb(t_2)$ and $S.lw(t_2,x) = t_1$.
	This is a contradiction.
%	
%	$t_1 [\textcolor{blue}{rf}^x] t_2$ gives us $\storeact(p,t_1) < \issueact(p,t_2)$.  Now, 
%	$t_3 [\textcolor{red}{po} \cup \textcolor{blue}{rf}]^+ t_2$ gives us 
%	a sequence
%	$\issueact(q, t_3) < \issueact(q,t^1_q) < \dots <\issueact(q,t^n_q)<\storeact(q,t^n_q) < \issueact(s,t^1_s)< \dots  < \issueact(s,t^m_s)< \storeact(r,t^m_s)<\issueact(r,t_1) < \storeact(p,t_1) < \issueact(p,t_2)$.  
%	
%By definition of 	$t_1 [\textcolor{blue}{rf}^x] t_2$, in the above $[\textcolor{red}{po} \cup \textcolor{blue}{rf}]^+$  chain of events starting with $\issueact(q, t_3)$ and ending in $\issueact(p,t_2)$, 
%$\issueact(r,t_1)$ is the last write that $t_2$ reads from. 
%This gives us $\issueact(q, t_3) <  \issueact(r,t_1)$, and hence $t_3 [\textcolor{orange}{co}^x] t_1$.  
\item Now we have to show that $(\textcolor{red}{po} \cup \textcolor{blue}{rf} \cup \textcolor{orange}{co})^+$ is acyclic. 
	
	It is clear that $\textcolor{red}{po}$ cannot generate cycles, since 
	it picks transactions in increasing order of their identifiers. Likewise, $\textcolor{orange}{co}$ is a total order, which is acyclic.
%	 Assume we have a  cycle  in $[\textcolor{red}{po} \cup \textcolor{blue}{rf}]^+$. This corresponds  to a sequence $\issueact(p,t) < \storeact(p,t)< \dots < \issueact(p,t)$. This contradicts  the third condition of legality 
%	in the execution summary which says that for every transaction $t$ and 
%	processes $p, p'$, $\issueact(p,t) < \storeact(p',t)$. 
%	
	Assume we have a cycle in $[\textcolor{red}{po} \cup \textcolor{blue}{rf}]^+$. 
	 % in $(\textcolor{red}{po} \cup \textcolor{orange}{co} \cup \textcolor{blue}{rf})$. 
	This corresponds to a sequence $\issueact(p,t) < \dots < \storeact(q,t) <  \issueact(q,t_1) <  \dots < \storeact(r,t_1) < \issueact(p,t)$. However this gives us 
	$\storeact(q,t) <  \issueact(q,t_1)$ as well as $\storeact(r,t_1) < 
	 	  \issueact(p,t) < \storeact(r,t)$. The last inequality comes from the third condition of a legal execution. 
	 However, this gives us 	  $\storeact(q,t) <  \issueact(q,t_1) $ and 
	 $\storeact(r,t_1) < \storeact(r,t)$ contradicting the second condition of legal execution summaries. 
	
Hence, $(\textcolor{red}{po} \cup \textcolor{blue}{rf} \cup \textcolor{orange}{co})^+$ is acyclic.

\end{enumerate}

\end{proof}
%%%%%%%%%%
\section{$\ccvt$ Consistency of Partial Traces}
\label{app:ccv-sat}

\subsection{Adding Coherence Edges}
For a trace $\tau = \langle \tran,\textcolor{red}{po},\textcolor{blue}{rf},\textcolor{orange}{co} \rangle $, a variable $x \in \mathcal{X}$, and a pair $(t, t') \in \tran^{w,x} \times \tran^{w,x}$, we define $\tau \odot ( t_1 , t_2 ) := (\tran, \textcolor{red}{po} \cup \textcolor{blue}{rf} \cup \textcolor{orange}{co}')$, where $\textcolor{orange}{co}' := \textcolor{orange}{co} \cup \{ (t_1,t_2) \}$.

We first give an alternative definition for fulfilled traces.

\begin{lemma}
 A trace $\tau=\langle \tran,\textcolor{red}{po},\textcolor{blue}{rf},\textcolor{orange}{co} \rangle $ is \emph{fulfilled} iff, 
   for all transactions $t, t' \in \tran^{w,x}$,  $t \neq t'$, 
           whenever 
    $t$ 
$[\textcolor{red}{po} \cup \textcolor{blue}{rf} \cup \textcolor{orange}{co}^x]^+ t''$ and $t' [\textcolor{blue}{rf}^x] t''$, then $t$ 
$[\textcolor{red}{po} \cup \textcolor{blue}{rf} \cup \textcolor{orange}{co}^x]^+ t'$.
\label{lem:ful}
\end{lemma}
\begin{proof}
Recall that we have defined a trace as fulfilled, if  for all transactions $t, t' \in \tran^{w,x}$,  $t \neq t'$, 
           whenever $t$ 
$[\textcolor{red}{po} \cup \textcolor{blue}{rf} ]^+ t''$ and $t' [\textcolor{blue}{rf}^x] t''$, then $t$ 
$[\textcolor{orange}{co}^x]^+ t'$. Now we show that 
the new condition in the lemma statement above implies this condition.

Show that the condition 

\begin{center}
	$t$ 
$[\textcolor{red}{po} \cup \textcolor{blue}{rf} \cup \textcolor{orange}{co}^x]^+ t''$ and $t' [\textcolor{blue}{rf}^x] t'' \Rightarrow t$ 
$[\textcolor{red}{po} \cup \textcolor{blue}{rf} \cup \textcolor{orange}{co}^x]^+ t'$ 
\end{center}
implies the condition 

\begin{center}

$t$ 
$[\textcolor{red}{po} \cup \textcolor{blue}{rf} ]^+ t''$ and $t' [\textcolor{blue}{rf}^x] t'' \Rightarrow t$ 
$[\textcolor{orange}{co}^x]^+ t'$. 
	
\end{center}

Assume
	$t$ 
$[\textcolor{red}{po} \cup \textcolor{blue}{rf} \cup \textcolor{orange}{co}^x]^+ t''$. This  means either 
\begin{itemize}
\item[(1)]	
 $t$ 
$[\textcolor{red}{po} \cup \textcolor{blue}{rf}]^+ t''$ (we do not have 
$\textcolor{orange}{co}^x$ edges from $t$ to $t''$), 
or 
\item[(2)] $t$ 
$[\textcolor{red}{po} \cup \textcolor{blue}{rf} \cup \textcolor{orange}{co}^x]^+ s [\textcolor{red}{po} \cup \textcolor{blue}{rf}]^+ t''$. 

\end{itemize}

\begin{itemize}
	\item[(a)]
Assume(1). Then we have  $t$ 
$[\textcolor{red}{po} \cup \textcolor{blue}{rf}]^+ t''$ and $t' [\textcolor{blue}{rf}^x] t''$. From the given condition we know 
$t$ 
$[\textcolor{red}{po} \cup \textcolor{blue}{rf} \cup \textcolor{orange}{co}^x]^+ t'$. By assumption, $\neg [t 
[\textcolor{red}{po} \cup \textcolor{blue}{rf} \cup \textcolor{orange}{co}^x]^+ t'']$.

%Hence, $t$ 
%$[\textcolor{red}{po} \cup \textcolor{blue}{rf} \cup \textcolor{orange}{co}^x]^+ t'$ should actually be 
% $t$ 
%$[\textcolor{orange}{co}^x]^+ t'$ (otherwise, we have 
%$t [\textcolor{red}{po} \cup \textcolor{blue}{rf} \cup \textcolor{orange}{co}^x]^+ t' [\textcolor{blue}{rf}^x] t''$ which will give $[t 
%[\textcolor{red}{po} \cup \textcolor{blue}{rf} \cup \textcolor{orange}{co}^x]^+ t'']$, contradicting $\neg [t 
%[\textcolor{red}{po} \cup \textcolor{blue}{rf} \cup \textcolor{orange}{co}^x]^+ t'']$). 

 Note that if we conclude 
$t$ 
$[\textcolor{red}{po} \cup \textcolor{blue}{rf} \cup \textcolor{orange}{co}^x]^+ t'$, then, with $t' [\textcolor{blue}{rf}^x] t''$, we will also get 
$t$ 
$[\textcolor{red}{po} \cup \textcolor{blue}{rf} \cup \textcolor{orange}{co}^x]^+ t''$, which by assumption (1) we do not. Thus, we have only $t$ 
$[ \textcolor{orange}{co}^x]^+ t'$. 

Thus we obtain $t$ 
$[\textcolor{red}{po} \cup \textcolor{blue}{rf}]^+ t''$ and $t' [\textcolor{blue}{rf}^x] t''$ gives $t$ 
$[\textcolor{orange}{co}^x]^+ t'$.

\item[(b)]Now consider condition (2), where we have $t$ 
$[\textcolor{red}{po} \cup \textcolor{blue}{rf} \cup \textcolor{orange}{co}^x]^+ s [\textcolor{red}{po} \cup \textcolor{blue}{rf}]^+ t''$, and $t' [\textcolor{blue}{rf}^x] t''$. From (1) above, using 
$s [\textcolor{red}{po} \cup \textcolor{blue}{rf}]^+ t''$, and $t' [\textcolor{blue}{rf}^x] t''$ we obtain $s$ 
$[\textcolor{orange}{co}^x]^+ t'$. Again, as in (1), 
if we allow only $t$ 
$[\textcolor{red}{po} \cup \textcolor{blue}{rf}]^+ t''$, then 
we need to have $t [\textcolor{orange}{co}^x]^+ s$; otherwise we 
will have $t$ 
$[\textcolor{red}{po} \cup \textcolor{blue}{rf} \cup \textcolor{orange}{co}^x]^+ s [\textcolor{red}{po} \cup \textcolor{blue}{rf}]^+ t''$. Hence, $t [\textcolor{orange}{co}^x]^+ s$ and $s$ 
$[\textcolor{orange}{co}^x]^+ t'$ gives $t [\textcolor{orange}{co}^x]^+ t'$.

\end{itemize}

\end{proof}

%%%%%
\begin{lemma}
If $\tau_1$ is fulfilled, $t_1$, $t_2 \in \tran^{w,x}$, $t_1 \ne t_2$ , and $\tau_2 = \tau_1 \odot (t_1,t_2)$ then $\tau_2$ is fulfilled.
\label{fulfilled-co-fulfilled}
\end{lemma}

\begin{proof}
    Let $\tau_1 = (\tran,\textcolor{red}{po},\textcolor{blue}{rf},\textcolor{orange}{co}_1)$, and $\tau_2 = (\tran,\textcolor{red}{po},\textcolor{blue}{rf},\textcolor{orange}{co}_2)$. Suppose that there are transactions $t_3$, $t_4$, and $t_5$ such that $t_3$ [$\textcolor{red}{po} \cup \textcolor{blue}{rf} \cup \textcolor{orange}{co}_2^x$]$^+$ $t_5$ and $t_4$ [$\textcolor{blue}{rf}^x$] $t_5$. We show that $t_3$ [$\textcolor{red}{po} \cup \textcolor{blue}{rf} \cup \textcolor{orange}{co}_2^x$]$^+$ $t_4$. We consider two cases.
    \begin{itemize}
    
     \item[(i)] $t_3$ [$ \textcolor{red}{po} \cup \textcolor{blue}{rf} \cup \textcolor{orange}{co}_1^x$]$^+$ $t_5$. Since $\tau_1$ is fulfilled, we will have $t_3$ [$\textcolor{red}{po} \cup \textcolor{blue}{rf} \cup \textcolor{orange}{co}_1^x$]$^+$ $t_4$. Since $\tau_1 \sqsubseteq \tau_2$ it follows that $t_3$ [$\textcolor{red}{po} \cup \textcolor{blue}{rf} \cup \textcolor{orange}{co}_2^x$]$^+$ $t_4$.
    
    \item[(ii)] $t_3 [  \textcolor{red}{po} \cup \textcolor{blue}{rf} \cup \textcolor{orange}{co}^{x}_1 $ ]$^+$ $t_1$ and $t_2$ [$\textcolor{red}{po} \cup \textcolor{blue}{rf} \cup \textcolor{orange}{co} _{1}^x$]$^+$ $t_5$. Note that we added $(t_1, t_2)$ as a new $co$ edge to obtain $\tau_2$.

    Since $\tau_1$ is fulfilled, $t_2$ [$\textcolor{red}{po} \cup \textcolor{blue}{rf} \cup \textcolor{orange}{co}_{1}^x$]$^+$ $t_4$. Moreover, $t_3$ [$\textcolor{red}{po} \cup \textcolor{blue}{rf} \cup \textcolor{orange}{co}_{1}^x$]$^+$ $t_1$ and $\tau_1 \sqsubseteq \tau_2$, so we have $t_3$ [$\textcolor{red}{po} \cup \textcolor{blue}{rf} \cup \textcolor{orange}{co}_{2}^x$]$^+$ $t_1$. Hence, we have $t_3$ [$\textcolor{red}{po} \cup \textcolor{blue}{rf} \cup \textcolor{orange}{co}_{2}^x$]$^+$ $t_1$ [$
    \textcolor{orange}{co}_{2}^x$] $t_2$ [$\textcolor{red}{po} \cup \textcolor{blue}{rf} \cup \textcolor{orange}{co}_{2}^x$]$^+$ $t_4$, i.e., we have $t_3$ [$\textcolor{red}{po} \cup \textcolor{blue}{rf} \cup \textcolor{orange}{co}_{2}^x$]$^+$ $t_4$.
    \end{itemize}

\end{proof}
%%%%%

%%%%%%%%%%%%%
\begin{lemma}
   Assume $\tau_1 = \langle \tran,\textcolor{red}{po},\textcolor{blue}{rf},\textcolor{orange}{co}_1 \rangle $ is fulfilled, $\tau_1 \models \ccvt$, %and  $[\prcn{1}$]$^+$ is acyclic, 
        and there exists $t_1$, $t_2$ $\in \tran^{w,x}$, such that 
    $\neg[t_2 (\textcolor{red}{po} \cup \textcolor{blue}{rf} \cup \textcolor{orange}{co}_1)^+ t_1]$. Then  $\tau_2 = \tau_1 \odot ( t_1,t_2) $ is such that  $\tau_2 \models \ccvt$.  
    %and      $[\prcn{2}$]$^+$ is acyclic. 
    \label{ccv-co-ccv}

\end{lemma}

\begin{proof}
Let $\tau_1 = \langle \tran,\textcolor{red}{po},\textcolor{blue}{rf},\textcolor{orange}{co}_1 \rangle $. Assume  we have a $[\prc]$ cycle in $\tau_2$ :  $t$ [$\textcolor{red}{po} \cup \textcolor{blue}{rf} \cup \textcolor{orange}{co}_2$]$^+$ $t$. Since $\tau_1$ is fulfilled, it follows from Lemma \ref{fulfilled-co-fulfilled} that $\tau_2$ is fulfilled. We consider two possible cases.
\begin{itemize}

\item[(i)] $t$ [$\prcn{1}$]$^+$ $t$. This contradicts the premise that $[\prcn{1}$]$^+$ is acyclic. 

\item[(ii)] $t$ [$\prcn{1}]^+ t_1 [\textcolor{orange}{co}_2^x$] $t_2 [\prcn{1}]^+t$. This means that $t_2$ [$\prcn{1}]^+ t_1$ which contradicts the premise that $\neg[t_2 (\textcolor{red}{po} \cup \textcolor{blue}{rf} \cup \textcolor{orange}{co}_1)^+ t_1]$.
	
\end{itemize}
Thus, $(\tpo \cup \trf \cup \tco_2)^+$ is acyclic. Now for the rest of the conditions to show that $\tau_2$ respects $\ccvt$. 
  
Assume that $\tau_2 \nvDash \ccvt$. Since $\tau_2$ is fulfilled by Lemma \ref{fulfilled-co-fulfilled}, the second condition for $\models \ccvt$
holds good. Assume that $\textcolor{orange}{co}_2^x;[\textcolor{red}{po} \cup \textcolor{blue}{rf}]^+$ is reflexive. Then we have $(t_1, t_2) \in  \textcolor{orange}{co}_2^x$, and $t_2 [\textcolor{red}{po} \cup \textcolor{blue}{rf}]^+ t_1$. This however contradicts our assumption 
that $\neg[t_2 (\textcolor{red}{po} \cup \textcolor{blue}{rf} \cup \textcolor{orange}{co}_1)^+ t_1]$. Hence $\tau_2 \models \ccvt$.

\end{proof}

%%%%%%%%%%
\subsection{Proof of Theorem \ref{ccv-sat}}
\begin{proof}
 Assume we have a fulfilled, partially good trace  $\tau=\langle \tran,\textcolor{red}{po},\textcolor{blue}{rf},\textcolor{orange}{co} \rangle $.
 By definition of partially good traces, we know that $\tau \models \ccvt$ and $(\textcolor{red}{po} \cup \textcolor{blue}{rf}\cup \textcolor{orange}{co})^+$ is acyclic. 
   To show that $\tau$ is $\ccvt$ consistent, we have to show that we can extend $\tau$ to a total, $\ccvt$ consistent trace $\tau'$. 
 
 For extending $\tau$, 
 we construct a sequence of traces $\tau=\tau_0 \sqsubseteq \tau_1 \sqsubseteq \tau_2,...$, such that 
 \begin{enumerate}
 	\item Each  $\tau_i = \langle \tran,\textcolor{red}{po},\textcolor{blue}{rf},\textcolor{orange}{co}_{i} \rangle$ is fulfilled,
 	\item $\tau_i \models \ccvt$
 \end{enumerate}
 
 If $\tau_i$ is not total, then we generate trace $\tau_{i+1} = \langle \tran,\textcolor{red}{po},\textcolor{blue}{rf},\textcolor{orange}{co}_{i+1} \rangle$, by adding $t$ $[\textcolor{orange}{co}]$ $t'$ to $\textcolor{orange}{co}_{i+1}$ for transactions $t$ and $t'$ which write on some same variable,  such that  $\neg(t'\,[\textcolor{red}{po} \cup \textcolor{blue}{rf}\cup \textcolor{orange}{co}_i]^+\,t)$ and $ \neg (t'\,[\textcolor{orange}{co}_i]\,t)$. As $\tau_i$ is fulfilled, $\tau_{i+1}$ is also fulfilled (Lemma \ref{fulfilled-co-fulfilled}). 
  Also,  $\tau_{i+1} \models \ccvt$ (Lemma \ref{ccv-co-ccv}).
   If $\tau_{i+1}$ is not total, then we generate trace $\tau_{i+2}$. We continue generating these new traces until we get a total trace $\tau_n$. We obtain $\tau_n$ which is total and 
   $\tau_n \models \ccvt$.     Hence, $\tau_n$ is $\ccvt$-consistent.

 So, we successfully extended $\tau$ to a $\ccvt$ consistent total trace $\tau_n$. Hence, $\tau$ is $\ccvt$ consistent. 
\end{proof}

%%%%%%%%%%%%%%%%%%%%%%%%%%%%%%%%%5

%%%%%%%%%%%%%%%%%%%%%%%%

\section{Properties of the Fulfilled Semantics}

\label{app:satcons}
%For traces $\tau_1 = \langle \tran_1, \textcolor{red}{po}_1, \textcolor{blue}{rf}_1, \textcolor{orange}{co}_1 \rangle$ and $\tau_2 = \langle \tran_2, \textcolor{red}{po}_2, \textcolor{blue}{rf}_2, \textcolor{orange}{co}_2 \rangle$, we say $\tau_1 \equiv \tau_2$ if $\tran_1 = \tran_2$, $\tpo_1 = \tpo_2$, $\trf_1 = \trf_2$ and for all $t_1$,$t_2 \in \tran_1^{w,x}$ we have $t_1$ [$\tpo_1 \cup \trf_1 \cup \tco_1^x$] $t_2$ iff $t_1$ [$\tpo_2 \cup \trf_2 \cup \tco_2^x$] $t_2$.
We show that all traces $\tau$ generated in the fulfilled semantics are (i) fulfilled, and (ii) $\tau \models \ccvt$, and therefore, 
by Theorem \ref{thm:ccv} are $\ccvt$ consistent. In particular, 
Lemma \ref{lem:f1}, \ref{lem:f2}, \ref{lem:f3} and \ref{lem:f4} imply Lemma \ref{lem:satcons}.

\begin{lemma}
	For traces $\tau_1$ and $\tau_2$ if $\tau_1$ $\xrightarrow[]{(begin,t)}_{\sat}$ $\tau_2$, and $\tau_1$ is fulfilled then $\tau_2$ is fulfilled.
	\label{lem:f1}
\end{lemma}

\begin{proof}
	Let $\tau_1 = \langle \tran_1, \textcolor{red}{po}_1 , \textcolor{blue}{rf}_1, \textcolor{orange}{co}_1 \rangle$ and $\tau_2 = \langle \tran_2, \textcolor{red}{po}_2, \textcolor{blue}{rf}_2, \textcolor{orange}{co}_2 \rangle$. 
Assume $\tau_1$ is fulfilled. By definition of $\xrightarrow[]{(begin,t)}_{\sat}$ it follows that $\tran_1 \subseteq \tran_2, \tpo_1 \subseteq \tpo_2$, $\trf_1 \subseteq \trf_2$, and $\tco_1 \subseteq \tco_2$.
Assume that $t_1$ [$\tpo_2 \cup \trf_2 \cup \tco_2$]$^+$ $t_2$, and 
 $t'$ [$\trf^y_2$]$ t_2$. The newly added transaction $t \in \tran_2$ has no successors  in $\tpo_2 \cup \trf_2 \cup \tco_2$, hence it follows that 
 $t_1$ [$\tpo_1 \cup \trf_1 \cup \tco_1$]$^+$ $t_2$ and  $t'$ [$\trf^y_1$]$ t_2$. As $\tau_1$ is fulfilled, we have $t_1$ [$\tpo_1 \cup \trf_1 \cup \tco_1$]$^+$ $t'$, and hence $t_1$ [$\tpo_2 \cup \trf_2 \cup \tco_2$]$^+$ $t'$.
Thus, $\tau_2$ is fulfilled whenever $\tau_1$ is. 

%
%for all transactions 
%$t_1 \neq t_2$, $t_1, t_2 \in \tran^w$ and all variables $x$, if we have 
%$t_1$ [$\tpo_1 \cup \trf_1$]$^+$ $t_2$, and 
% $t'$ [$\trf^x_1$]$ t_2$, we have $t_1 [\tco_1^x] t'$. The transition on $t$
% means that we are seeing a  $\beginact(p,t)$ instruction which results in 
% $\tran_2=\tran_1 \cup \{t\}, \textcolor{red}{po}_2= \textcolor{red}{po}_1 \cup (t',t) $ where $t'$ is the last transaction executed in $p$, and the other relations 
% remain the same. In particular, $\textcolor{orange}{co}_2=\textcolor{orange}{co}_1$ and 
% $\textcolor{blue}{rf}_2=\textcolor{blue}{rf}_1$.
% Then indeed we have 
% 	 for all transactions 
%$t_1 \neq t_2$, $t_1, t_2 \in \tran^w$ and all variables $x$, if we have 
%$t_1$ [$\tpo_2 \cup \trf_2$]$^+$ $t_2$, and 
% $t'$ [$\trf^x_2$]$ t_2$, we have $t_1 [\tco_2^x] t'$.
%	
%	
%	By definition of  $\tau_1 \equiv \tau_2$ it follows that $\tran_1 \subset \tran_2$, $\tpo_1 \subset \tpo_2$, $\trf_1 \subset \trf_2$, and $\tco_1 \subset \tco_2$. Assume that $t_1$ [$\tpo_2 \cup \trf_2 \cup \tco_2^x$]$^+$ $t_3$ and $t_2$ [$\trf_2^x$] $t_3$. We show that $t_1$ [$\tpo_2 \cup \trf_2 \cup \tco_2^x$]$^+$ $t_2$. Transition $\tau_1 \equiv \tau_2$ does not add new $\trf$ and $\tco$ relations and $t$ does not have successor in $\tpo_2 \cup \trf_2 \cup \tco_2$, it follows that $t_1$ [$\tpo_1 \cup \trf_1 \cup \tco_1^x$]$^+$ $t_3$ and $t_2$ [$\trf_2^x$] $t_3$.  $\tau_1$ is fulfilled, we will have $t_1$ [$\tpo_1 \cup \trf_1 \cup \tco_1^x$]$^+$ $t_2$, and hence $t_1$ [$\tpo_2 \cup \trf_2 \cup \tco_2^x$]$^+$ $t_2$.
\end{proof}
%%%%%%%%%%%%%%%%%%%%%
\begin{lemma}
	For traces $\tau_1$ and $\tau_2$ if $\tau_1$ $\xrightarrow[]{(read,t,t')}_{\sat}$ $\tau_2$, and $\tau_1$ is fulfilled then $\tau_2$ is fulfilled.
	\label{lem:f2}
\end{lemma}
\begin{proof}
    Let $\tau_1 = \langle \tran_1 , \textcolor{red}{po}_1 , \textcolor{blue}{rf}_1, \textcolor{orange}{co}_1 \rangle$, $\tau_2 = \langle \tran_2, \textcolor{red}{po}_2, \textcolor{blue}{rf}_2, \textcolor{orange}{co}_2 \rangle$. Let $ev = r(p,t,x,v)$ be the read event in $t$, and let  $t' \in \rbl(\tau,t,x)$ be the chosen transaction that $t$ reads from, while $\tau_1$ $\xrightarrow[]{(read,t,t')}_{\sat}$ $\tau_2$. Then 
    $\tran_2=\tran_1$, $\textcolor{blue}{rf}_2=\textcolor{blue}{rf}_1 \cup (t',t)$, $\textcolor{orange}{co}_2=\textcolor{orange}{co}_1 
    \cup \{(t'',t') \mid t'' \in \vbl(\tau,t,x)\} \cup \{(t',t_2) \mid 
    t' \in \tran_1^{w,y}$, and $t_2 [\textcolor{blue}{rf}]^y_2 t\} 
    $. Assume  for any two transactions $t_1, t_2$ and any variable $y$,  
        $t_1$ [$\tpo_2 \cup \trf_2 \cup \tco_2^y$]$^+$ $t_3$ and $t_2$ [$\trf_2^y$] $t_3$. We show that $t_1$ [$\tpo_2 \cup \trf_2 \cup \tco_2^y$]$^+$ $t_2$. Since $t$ has no successors in $\tpo_2 \cup \trf_2 \cup \tco_2$, we only need to consider the following cases.
            \begin{itemize}
        \item [$\bullet$] $y$ = $x$, $t_3 = t$, $t_2 = t'$ 
%        Then we have  $t_1$ [$\tpo_2 \cup \trf_2 \cup \tco_2^x$]$^+$ $t$ and $t'$ [$\trf_2^x$] $t$.
and there is a transaction $t_4 \in \vbl(\tau,t,x)$ such that $t_1$ [$\tpo_1 \cup \trf_1 \cup \tco_1^x$]$^*$ $t_4$. 
        From the definition of $\xrightarrow[]{(read,t,t')}_{\sat}$, we  have $t_4$ [$\tco_2^x$] $t_2$. Since $t_1$ [$\tpo_1 \cup \trf_1 \cup \tco_1^x$]$^*$ $t_4$, we also have $t_1$ [$\tpo_2 \cup \trf_2 \cup \tco_2^x$]$^*$ $t_4$. So we have 
        $t_1$ [$\tpo_2 \cup \trf_2 \cup \tco_2^x$]$^+$ $t_4$ [$\tco_2^x$] $t_2$.
        \item [$\bullet$] $y=x$ and there is a transaction $t_4 \in \vbl(\tau,t,x)$. By definition of $\xrightarrow[]{(read,t,t')}_{\sat}$ we have $t_4$ [$\tco_2^x$] $t'$.

        By assumption we have 
    $t_1$ [$\tpo_2 \cup \trf_2 \cup \tco_2^x$]$^+$ $t_3$ and $t_2$ [$\trf_2^x$] $t_3$. Indeed $t_2$ [$\trf_1^x$] $t_3$, since the only new $\trf$ added to $\tau_2$ is $(t',t)$.   
    We do not have $t_1$ [$\tpo_1 \cup \trf_1 \cup \tco_1^x$]$^+$ $t_3$, since otherwise along with  $t_2$ [$\trf_1^x$] $t_3$ and the fulfilledness of $\tau_1$ will result in $t_1$ [$\tpo_1 \cup \trf_1 \cup \tco_1^x$]$^+$ $t_2$ and hence $t_1$ [$\tpo_2 \cup \trf_2 \cup \tco_2^x$]$^+$ $t_2$.

       Thus, $t_1$ [$\tpo_2 \cup \trf_2 \cup \tco_2^x$]$^+$ $t_3$ is obtained 
       using the new $t_4 [\tco_2^x] t'$ edge 
        as $t_1$ [$\tpo_1 \cup \trf_1 \cup \tco_1^x$]$^*$ $t_4 [\tco_2^x] t'$ [$\tpo_1 \cup \trf_1 \cup \tco_1^x$]$^+$ $t_3$.

        We know that $\tau_1$ is fulfilled, and we also have $t_2$ [$\trf_2^y$] $t_3$. Together with $t'$ [$\tpo_1 \cup \trf_1 \cup \tco_1^x$]$^+$ $t_3$, this gives the following. 
        \begin{enumerate}
        	\item either  $t_2$ [$\trf_1^y$] $t_3$ assuming $\neg(t_2=t' \wedge t_3=t)$, in which case the fulfilled status of $\tau_1$ gives 
                        $t'$ [$\tpo_1 \cup \trf_1 \cup \tco_1^x$]$^+$ $t_2$ i.e. $t'$ [$\tpo_2 \cup \trf_2 \cup \tco_2^x$]$^+$ $t_2$, 
       \item  $\neg$($t_2$ [$\trf_1^y$] $t_3$). Then 
                        $t_2$ [$\trf_2^y$] $t_3$ is the new reads from introduced, which means $t_2=t', t_3=t$. This is already handled by the above bullet. So we again have  $t'$ [$\tpo_1 \cup \trf_1 \cup \tco_1^x$]$^+$ $t_2$ and hence $t'$ [$\tpo_2 \cup \trf_2 \cup \tco_2^x$]$^+$ $t_2$. 
              \end{enumerate}
                      
               Since $t_1$ [$\tpo_1 \cup \trf_1 \cup \tco_1^x$]$^*$ $t_4$ and $t'$ [$\tpo_1 \cup \trf_1 \cup \tco_1^x$]$^+$ $t_3$, it follows that $t_1$ [$\tpo_2 \cup \trf_2 \cup \tco_2^x$]$^*$ $t_4$ and $t' [\tpo_2 \cup \trf_2 \cup \tco_2^x$]$^+$ $t_3$. That is, we have $t_1$ [$\tpo_2 \cup \trf_2 \cup \tco_2^x$]$^*$ $t_4$  [$\tco_2^x$] $t'$ [$\tpo_2 \cup \trf_2 \cup \tco_2^x$]$^+$ $t_2$. Hence $t_1$ [$\tpo_2 \cup \trf_2 \cup \tco_2^x$]$^+$ $t_2$.
%        
%        
%        
%        [$\tco_2^y$] $t'$ [$\tpo_2 \cup \trf_2 \cup \tco_2^y$]$^+$ $t_2$, i.e., $t_1$ [$\tpo_2 \cup \trf_2 \cup \tco_2^y$]$^+$ $t_2$.
        \item [$\bullet$] $y \neq x$. By assumption, we have $t_1$ [$\tpo_2 \cup \trf_2 \cup \tco_2^y$]$^+$ $t_3$ and $t_2$ [$\trf_2^y$] $t_3$. We show that $t_1$ [$\tpo_2 \cup \trf_2 \cup \tco_2^y$]$^+$ $t_2$.
     Note that  the only new $\trf_2$ added to $\tau_2$ is $(t',t)$, hence we also have
     $t_2$ [$\trf_1^y$] $t_3$. Indeed we do not have $t_1$ [$\tpo_1 \cup \trf_1 \cup \tco_1^y$]$^+$ $t_3$ : else the fulfilled status of $\tau_1$ will already give us $t_1$ [$\tpo_1 \cup \trf_1 \cup \tco_1^y$]$^+$ $t_2$
            and hence $t_1$ [$\tpo_2 \cup \trf_2 \cup \tco_2^y$]$^+$ $t_2$.

   \smallskip 
        
         Assume there is a transaction $t_4$ such that $t_4$ [$\trf_1^y$] $t$, $y \neq x$, and let $t' \in \rbl(\tau,t,x)$ be such that 
                  $t' \in \tran_1^{w,y} \cap \tran^{w,x}$.   Now by the definition of  $\xrightarrow[]{(read,t,t')}_{\sat}$, $t' \in  \tran_1^{w,y} $ and $t_4$ $[\textcolor{blue}{rf}_1]^y t$   gives          $(t',t_4) \in [\textcolor{orange}{co}_2]^y$. 
    \smallskip              
                  
    By assumption, we have $t_1$ [$\tpo_2 \cup \trf_2 \cup \tco_2^y$]$^+$ $t_3$. Since we did not have 
    $t_1$ [$\tpo_1 \cup \trf_1 \cup \tco_1^y$]$^+$ $t_3$, using 
    $t' [\textcolor{orange}{co}_2]^y t_4 
        $, we can obtain $t_1$ [$\tpo_2 \cup \trf_2 \cup \tco_2^y$]$^+$ $t_3$ as follows :
      $t_1$ [$\tpo_1 \cup \trf_1 \cup \tco_1^y$]$^*$ $t' [\textcolor{orange}{co}_2]^y t_4 
        $ [$\tpo_1 \cup \trf_1 \cup \tco_1^y$]$^+$ $t_3$.  We have $t_2$ [$\trf_2^y$] $t_3$, which gives $t_2$ [$\trf_1^y$] $t_3$, since the only new $\trf_2$ added is $(t',t)$.

      The fulfilled status of $\tau_1$ along with 
                  $t_4$ [$\tpo_1 \cup \trf_1 \cup \tco_1^y$]$^+$ $t_3$ and 
                  $t_2$ [$\trf_1^y$] $t_3$ gives $t_4$ [$\tpo_1 \cup \trf_1 \cup \tco_1^y$]$^+$ $t_2$.     Then we have 
        $t_1$ [$\tpo_2 \cup \trf_2 \cup \tco_2^y$]$^*$ $t'$  [$\tco_2^y$] $t_4$ [$\tpo_1 \cup \trf_1 \cup \tco_1^y$]$^+$ $t_2$. This gives us 
         $t_1$ [$\tpo_2 \cup \trf_2 \cup \tco_2^y$]$^+$ $t_2$.

%        Since $\tau_1$ is fulfilled, $t_4$ [$\tpo_1 \cup \trf_1 \cup \tco_1^y$]$^+$ $t_3$ and $t_2$ [$\trf_1^y$] $t_3$ gives 
%        $t_4$ [$\tpo_1 \cup \trf_1 \cup \tco_1^y$]$^+$ $t_2$. 
%        
%         
%        
%        
%        
%        we will have $t'$ [$\tpo_1 \cup \trf_1 \cup \tco_1^y$]$^+$ $t_2$. Moreover, $t$ has no successor in $\tpo_2 \cup \trf_2 \cup \tco_2$, hence it follows that $t_1$ [$\tpo_2 \cup \trf_2 \cup \tco_2^y$]$^*$ $t'$, and $t'$ [$\tpo_2 \cup \trf_2 \cup \tco_2^y$]$^+$ $t_2$. From the definition of $\xrightarrow[]{(ev,t')}_{\sat}$, we will have $t'$ [$\tco_2$] $t_4$. Hence we get, $t_1$ [$\tpo_2 \cup \trf_2 \cup \tco_2^y$]$^*$ $t'$ [$\tco_2^y$] $t_4$ [$\tpo_2 \cup \trf_2 \cup \tco_2^y$]$^+$ $t_3$, i.e. $t_1$ [$\tpo_2 \cup \trf_2 \cup \tco_2^y$]$^+$ $t_2$.

    \end{itemize}
\end{proof}
%%%%%%%%%%%%%%%%%
\begin{lemma}
    If $\tau_1 \models \ccvt$  and $\tau_1$ $\xrightarrow[]{(begin,t)}_{\sat}$ $\tau_2$ then $\tau_2 \models \ccvt$.
    \label{lem:f3}
\end{lemma}
\begin{proof}
The proof follows trivially since we do not change the  	reads from and coherence order relations, and the transaction $t$ added to the partial order has no successors. Thus, if $\tau_1 \models \ccvt$, 
so does $\tau_2$.  
	\end{proof}

%%%%%%%%%%%%%%%%%
\begin{lemma}
    If $\tau_1 \models \ccvt$  and $\tau_1$ $\xrightarrow[]{(read,t,t')}_{\sat}$ $\tau_2$ then $\tau_2 \models \ccvt$.
    \label{lem:f4}
\end{lemma}

\begin{proof}
    Let $\tau_1 = \langle \tran_{1} , \textcolor{red}{po}_1 , \textcolor{blue}{rf}_1, \textcolor{orange}{co}_1 \rangle$, $\tau_2 = \langle \tran_{2} , \textcolor{red}{po}_2 , \textcolor{blue}{rf}_2, \textcolor{orange}{co}_2 \rangle$, and $ev$ = $r(p,t,x,v)$ be a read event in transaction $t \in \tran_1$. Suppose $\tau_2 \nvDash \ccvt$, and  that $\tpo_2 \cup \trf_2 \cup \tco_2$ is cyclic. Since $\tau_1 \models \ccvt$, and $t$ has no outgoing edges, 
   on adding $(t',t) \in \textcolor{blue}{rf}_2$, 
    it follows that the cycle in $\tau_2$ is as a result 
    of the newly added $\textcolor{orange}{co}_2$ edges. 
    
    We prove that 
    on adding $(t',t) \in \textcolor{blue}{rf}_2$, 
        such cycles are possible iff at least one of ${\tt{cond}_1}, \dots, {\tt{cond}_4}$ are true. 
    
 \subsection*{${\tt{cond1}}\vee \dots \vee {\tt{cond4}}$ induces $\tpo_2 \cup \trf_2 \cup \tco_2$ cyclicity }
   \label{sec:cyc1}
    This direction is easy to see : assume 
    one of ${\tt{cond1}}, \dots, {\tt{cond4}}$ are true; then, as already 
    argued in the main paper, we will get a $\tpo_2 \cup \trf_2 \cup \tco_2$ cycle on adding the $\textcolor{blue}{rf}_2$ edge from $t'$ to $t$ and we are done.

 \subsection*{$\tpo_2 \cup \trf_2 \cup \tco_2$ cyclicity implies ${\tt{cond1}}\vee \dots \vee {\tt{cond4}}$ }
 \label{sec:cyc2}
  For the converse direction, assume that we add the $\textcolor{blue}{rf}_2$ edge from $t'$ to $t$ and obtain a $\tpo_2 \cup \trf_2 \cup \tco_2$ cycle in $\tau_2$. We now argue that this cycle has been formed because one of 
 ${\tt{cond}_1}, \dots, {\tt{cond}_4}$ are true.  
 
 First of all, note that $t$ has no outgoing edges in $\tau_2$, since 
 it is the current transaction being executed. Also, 
 we know that $\tau_1$ has no $\tpo_1 \cup \trf_1 \cup \tco_1$ cycles. 
 Thus, the cyclicity of $\tpo_2 \cup \trf_2 \cup \tco_2$ is induced by the 
 newly added $\trf_2$ edge as well as the newly added 
  $\tco_2$ edges. Note that adding the $\trf_2$ edge  to $\tau_1$ does not induce any cycle since $t$ has no outgoing edges. Lets analyze the 
  $\tco_2$ edges added which induce cycles, and argue that 
  one of ${\tt{cond1}}, \dots, {\tt{cond4}}$ will be true.   
  
  \begin{enumerate}
  	\item We add  $\tco_2$ edges from $t'' \in \rbl(\tau_1, t,x)$ to $t'$. 
  	For  these edges to induce a cycle, we should have a path from $t'$ to $t''$ in $\tau_1$. That is, we have $t' [\tpo_1 \cup \trf_1 \cup \tco_1]^+ t''$. This is captured by ${\tt{cond1}}$.  
  	
  	\item Consider $y \neq x$. If $t' \in \tran^{w,x} \cap \tran^{w,y}$, 
  	and we have $t'''\textcolor{blue}{rf}_1^y t$.  Then we add 
  	$(t',t''') \in \tco^y_2$. To get a cycle, we need a path from 
  	$t'''$ to $t'$. 
  	\begin{itemize}
  	\item If $t''' \in \tran^{w,x} \cap \tran^{w,y}$, then we add $(t''', t') \in \tco^x_2$, resulting in a cycle. This is handled by  ${\tt{cond2}}$.
  	\item If we have a path 
  	$t''' [\tpo_1 \cup \trf_1 \cup \tco_1]^+ t'$, then we get a cycle again. This is handled by ${\tt{cond3}}$. 
  \item As a last case, to obtain a path from $t'''$ to $t'$, 
  assume there is a path from $t'''$ to $t$ in $\tau_1$, and let $t'' \in \tran^{w,x}$ be the last transaction writing to $x$ in this path.  Note that this will induce a path from $t'''$ to $t''$ to $t'$ : the path  from $t''$ to $t'$ comes by the $\tco^x_2$ edge added from $t''$ to $t'$ since 
  we have $(t',t) \in \trf_2^x$. Once we get this path from $t'''$ to $t'$, we again have the path we were looking for to get the cycle. This is handled by ${\tt{cond4}}$. 
    		
  	\end{itemize}
Thus, we have shown that obtaining a path from $t'''$ to $t'$ is covered 
by the conditions  ${\tt{cond}_1}, \dots, {\tt{cond}_4}$, and hence, 
a $\tpo_2 \cup \trf_2 \cup \tco_2$ cycle.  
  	  \end{enumerate}
 
 Thus, we can think of  $\tpo_2 \cup \trf_2 \cup \tco_2$ cycles as a result of the forbidden patterns described in ${\tt{cond}_i}$ $1 \leq i \leq 4$.  By construction of $\tau_1$ $\xrightarrow[]{(read,t,t')}_{\sat}$ $\tau_2$, we ensure $\neg {\tt{cond}_1}, \dots, \neg {\tt{cond}_4}$. Hence, 
    $\tau_2 \models \ccvt$.

\end{proof}

\section{Efficiency of Computing Readable and Visible Sets}
\subsection{Proof of Lemma \ref{lemma:poly}}
\label{app:poly}
%%%%
\begin{proof}
    We prove that set $\rbl(\tau, t, x)$ can be computed in polynomial time, by designing an algorithm to generate set $\rbl(\tau, t, x)$. The algorithm consists of the following  steps:
    \begin{itemize}
        \item[(i)] First we compute the  transitive closure of the relation 
        $[\tpo \cup \trf \cup \tco]$, i.e, we compute $[\tpo \cup \trf \cup \tco ]^+$.  We can use the Floyd-Warshall algorithm \cite{10.5555/1614191} to compute the transitive closure. This will take $O(|\tran|^3)$ time.
        \item[(ii)] We compute the set $\tran'=\{t'\mid t' [\tpo \cup \trf]^* t\}$. This takes $O(|\tran|^2)$ time.
        \item[(iii)] We compute the set $\tran''=\{t'\mid  t' \in \tran' \wedge \neg(\exists t'' . ( t' [\tpo \cup \trf \cup \tco]^* t'')) \}$. It takes $O(|\tran|^2)$ time.
        \item[(iv)] For each transaction $t' \in \tran^{w,x}$, we perform following checks:
        \begin{itemize}
            \item Check $\mathtt{cond 1 :} $ Check whether there exists a transaction $t'' \in \tran' \cap \tran^{w,x}$            
            with $t'$ $[\tpo  \cup \trf \cup \tco]^+$ $t''$. 
            If there is no such $t''$ then proceed to $\mathtt{cond 2}$. 
            If we find such $t''$, then $t' \notin \rbl(\tau , t, x)$. 
            This step will take $O(|\tran|^2)$ time.
            \item Check $\mathtt{cond 2 :}$ Check whether there exists a transaction $t''$ such that $t'' [\trf^y] t$ and $t',t'' \in \tran^{w,x} \cap \tran^{w,y}$. 
            If there is no such $t''$ then proceed to $\mathtt{cond 3}$. 
            If we find such $t''$, then $t' \notin \rbl(\tau , t, x)$. 
            This step will take $O(|\tran|)$ time.
            \item Check $\mathtt{cond 3 :}$ 
            
            We first check case 1 of $\mathtt{cond 3}$. Check whether there exists a transaction $t''$ such that $t'' [\trf^y] t$ , $t' \in \tran^{w,y}$, and $t'' [\tpo \cup \trf \cup \tco]^+ t'$. 
            If there is no such $t''$ then proceed to case two of $\mathtt{cond 3}$. 
            If we find such $t''$, then $t' \notin \rbl(\tau , t, x)$. 
            This step will take $O(|\tran|)$ time.
            
             Next, we  check case 2 of $\mathtt{cond 3}$. Check whether there are transactions $t''$ and $t'''$ such that $t'' [\trf^y] t$, $t''' \in \tran^{w,y}$, $t''' [\tpo \cup \trf \cup \tco]^+ t'$ and $t'' [\tpo \cup \trf \cup \tco]^+ t'''$. 
            If there are no such $t''$ and $t'''$ then proceed to $\mathtt{cond 4}$. 
            If we find such $t''$ and $t'''$, then $t' \notin \rbl(\tau , t, x)$. 
            This step will take $O(|\tran|^2)$ time.
            \item Check $\mathtt{cond 4 :}$ Check whether there are transactions $t''$ and $t'''$ such that $t'' [\trf^y] t$, $t''' \in \tran''$ and $t'' [\tpo \cup \trf \cup \tco]^+ t'''$. 
            If we find such $t''$ and $t'''$, 
            then $t' \notin$ $\rbl(\tau , t, x)$. 
            If there are no such $t''$ and $t'''$ then add $t'$ to $\rbl(\tau , t, x)$.
            This step will take $O(|\tran|^2)$ time.
        \end{itemize}
    \end{itemize}
    Similarly, we can compute $\vbl(\tau, t, x)$ in polynomial time. This completes the proof.
\end{proof}

%%%%%%%%%%%%%%%%%%%%%
\section{Incremental Total Semantics}
\label{app:inc}
In this section, we show that the weakenings of traces generated 
by the fulfilled semantics coincide with the  weakenings of $\ccvt$ consistent traces. To this end, we introduce a new \emph{incremental} semantics 
that is equivalent to the total $\ccvt$ semantics.
The \textit{incremental semantics} derives the total, $\ccvt$ consistent traces in an incremental fashion, step by step, and is used in the proof of Theorem \ref{thm:ccv}. 
%%%%%%%%%%%%%%%%%%%%%%%%%%%%%%%%%%%%%%%%%%%%%%%%%%%

\smallskip 

The \textit{incremental semantics} is given as the transition relation $\xrightarrow[]{}_{\inc}$ on pairs of configurations and traces, defined as  
$(\sigma,\tau) \xrightarrow[]{\alpha}_{\inc} (\sigma',\tau')$. The label $\alpha$ is one of the following (i) a begin transaction $(begin,t)$, (ii) a  $(write,t)$ corresponding to a  write event $w(p,t,x,v)$ in $t$, (iii) a triple $(read,t,t')$ corresponding to a read event $r(p,t,x,v)$ in transaction $t$, and  transaction $t'$ which $t$ reads from, and 
(iv) an end transaction $(end,t)$.  The transitions are described below.

\begin{itemize}
	\item [$\bullet$] Transition $(\sigma,\tau) \xrightarrow[]{(begin,t)}_{\inc} (\sigma',\tau')$ represents extending a total trace after visiting a $\beginact(p,t)$ event. Here, $\tau=\langle \tran,\tpo,\trf,\tco \rangle $, $\tau'=\langle \tran',\tpo',\trf',\tco' \rangle $, $\tran'= \tran \cup \{t\}$ and $\tpo' = \tpo \cup \{(t',t)\mid  t'$ is the last transaction  from $p$ which has been executed$\}$. 
	\item [$\bullet$] Transition $(\sigma,\tau) \xrightarrow[]{(write,t)}_{\inc} 	   (\sigma',\tau')$, where $ev = w(p,t,x,v)$, $\tau=\langle \tran,\tpo,\trf,\tco \rangle $, $\tau'=\langle \tran',\tpo',\trf',\tco' \rangle $, $\tran'= \tran$, $\tpo' =\tpo$, $\trf'=\trf$, $\tco \subseteq \tco'$ and $\tco'$ is a total order, describing  how to extend the total trace $\tau$ after visiting the write event $ev$ in transaction $t$, on variable $x$.
	\item [$\bullet$] Transition $(\sigma,\tau) \xrightarrow[]{(read,t,t')}_{\inc} 	   (\sigma',\tau')$ represents extending the total trace $\tau$ after visiting a read event $ev = r(p,t,x,v)$ in transaction $t$, and  $t$  reads from transaction $t'$. Here, $\tau=\langle \tran,\tpo,\trf,\tco \rangle $, $\tau'=\langle \tran',\tpo',\trf',\tco' \rangle $, $\tran'= \tran$, $\tpo' =\tpo$, $\trf'=\trf \cup \{(t',t)\}$, $\tco' = \tco$.
	\item [$\bullet$] Transition $(\sigma,\tau) \xrightarrow[]{(end,t)}_{\inc} 	   (\sigma',\tau')$, where $\sigma' = \sigma$, and $\tau' = \tau$ describes extendind trace after visiting end event.
\end{itemize}
   We define $\big[[\sigma]\big]^{\inc}$ = $\{ \tau \mid \exists \sigma' . \langle \sigma,\tau_{\o} \rangle \xrightarrow[]{*}_{\inc} \langle \sigma',\tau \rangle \}$as the set of traces generated according to the \textit{incremental semantics} starting from configuration $\sigma$ and the empty trace $\tau_{\o}$. We define $\big[[\sigma]\big]_{\ccvt}^{\inc}$ = $\big[[\sigma]\big]^{\inc}$ $\cap$ $\{ \tau | \tau$ is $\ccvt$ consistent$\}$. That is, it is the set of total traces $\tau$ such that   $\tau \models \ccvt$, generated by runs according to the incremental semantics starting from configuration $\sigma$  and the empty 
   trace. 
   
  \smallskip
  
  Starting from a configuration $\sigma$, for each run in the total $\ccvt$ semantics  leading to a trace $\tau=(\tran,  \tpo,\trf,\tco)$ there is a corresponding run $\big[[\sigma]\big]_{\ccvt}^{\inc}$ in the incremental semantics where the events are scheduled according to the relations $\tpo,\trf,\tco$, and conversely. Hence we obtain  
   
   \begin{lemma}
   	$\big[[\sigma]\big]_{\ccvt}^{\inc}$ = $\big[[\sigma]\big]_{\ccvt}$.
\label{lem:sim}
   \end{lemma}

  %%%%%%%%%%%%%%%%%%%%%%%%%%%%%%%%%%%%%%%%%%%%%%%%%%%
\section{Soundness of the DPOR Algorithm}
\label{app:thm:ccv}
We prove Theorem \ref{thm:ccv} below. 

\subsection{Proof of Theorem \ref{thm:ccv} }
We prove the two directions in the coming two subsections. 
First, in section \ref{app:dir1}, we show that all the weakenings of fulfilled  traces are also the weakenings of $\ccvt$ consistent traces. Then, in section \ref{app:dir2}, we show the converse direction, namely, weakenings of $\ccvt$ consistent traces are also weakenings of fulfilled traces.

%
%\noindent{\bf{Notations in the Fulfilled Semantics}}. 
%Recall that in the fulfilled semantics, we had transitions 
% $\xrightarrow[]{t}_{\sat}$ corresponding to a $\beginact(p,t)$ 
%instruction,   $\xrightarrow[]{(t,t')}_{\sat}$ corresponding to 
%a read event in transaction $t$, reading from $t'$. There were no transitions corresponding to write or ${\tt{end}}(p,t)$ instructions since there was no change in the state $(\sigma, \tau)$. 
%
%For convenience, in the following proof, we use transitions 
%   $(\sigma,\tau)\xrightarrow[]{(end,t)}_{\sat}(\sigma,\tau)$ to denote the end transaction events in the fulfilled semantics. To be symmetric with $\xrightarrow[]{(end,t)}_{\sat}$, we 
%  represent $(\sigma,\tau)\xrightarrow[]{t}_{\sat}(\sigma',\tau')$ corresponding to $\beginact(p,t)$ as
%  $(\sigma,\tau)\xrightarrow[]{(begin,t)}_{\sat}(\sigma',\tau')$. Likewise, we represent read and write events as 
%  $(\sigma,\tau)\xrightarrow[]{(read,t,t')}_{\sat}(\sigma',\tau')$ and $(\sigma,\tau)\xrightarrow[]{(write,t)}_{\sat}(\sigma,\tau)$. 
% This way, we have the same notations for the transitions in  $\xrightarrow[]{}_{\sat}$ and $\xrightarrow[]{}_{\inc}$. 

\subsection{$\{ weak(\tau) | \tau \in \big[[ \sigma]\big]_{\ccvt}^{\sat} \} \subseteq \{ weak(\tau) | \tau \in \big[[ \sigma]\big]_{\ccvt} \}$}
\label{app:dir1}

\begin{lemma}

If $(\sigma,\tau_1) \xrightarrow[]{(begin,t)}_{\sat} (\sigma',\tau_2)$, $\tau_2 \sqsubseteq \tau_4$, and $\tau_4$ is total then there exists a $\tau_3$ such that $(\sigma,\tau_3) \xrightarrow[]{(begin,t)}_{\inc} (\sigma',\tau_4)$ and $\tau_1 \sqsubseteq \tau_3$.
\label{lem:begin}
\end{lemma}

\begin{proof}
Let $\tau_1= \langle \tran_1,\tpo_1,\trf_1,\tco_1 \rangle$, $\tau_2= \langle \tran_2,\tpo_2,\trf_2,\tco_2 \rangle$, and $\tau_4= \langle \tran_4,\tpo_4,\trf_4, \tco_4 \rangle$. By definition of $\xrightarrow[]{(begin,t)}_{\sat}$, we have $\tran_2 = \tran_1$, $\tpo_2 = \tpo_1 \cup \{(t',t) \mid $ $t'$ is the last transaction executed in process $p\}$, 
 $\trf_2 = \trf_1$, and $ \tco_2 = \tco_1$. Since $\tau_2 \sqsubseteq \tau_4$ it follows that $\tran_4 = \tran_2$, $\tpo_4 = \tpo_2$, $\trf_4 = \trf_2$, and $ \tco_2 \subseteq \tco_4$.\\
Define $\tau_3 = \langle \tran_3,\tpo_3,\trf_3,\tco_3 \rangle$ such that $\tran_3 = \tran_1$, $\tpo_3 = \tpo_1$, $\trf_3 = \trf_1$, and $\tco_3 = 
\tco_4|_{\tran_3}$, is the order $\tco_4$ restricted to $\tran_3$.
 It follows that $(\sigma,\tau_3) \xrightarrow[]{(begin,t)}_{\inc} (\sigma',\tau_4)$. We need to show that $\tco_1 \subseteq \tco_3$. Consider $t$ [$\tco_1$] $t'$. It follows that $t$ [$\tco_2$] $t'$ and hence $t$ [$\tco_4$] $t'$. Since $t, t' \in \tran_1$, $\tco_3 = 
\tco_4|_{\tran_3}$, and $\tran_3=\tran_1$, we have $t$ [$\tco_3   $] $t'$.  
\end{proof}

\begin{lemma}
If $(\sigma,\tau_1) \xrightarrow[]{(write,t)}_{\sat} (\sigma',\tau_2)$, $\tau_2 \sqsubseteq \tau_4$, and $\tau_4$ is total then there exists a $\tau_3$ such that $(\sigma,\tau_3) \xrightarrow[]{(write,t)}_{\inc} (\sigma',\tau_4)$ and $\tau_1 \sqsubseteq \tau_3$.
\label{lem:wr}
\end{lemma}
\begin{proof}
This follows trivially  by the definition of the fulfilled semantics  	$\xrightarrow[]{(write,t)}_{\sat}$. Note that $\sigma=\sigma'$, 
and $\tau_1=\tau_2$. Hence, 
one can choose $\tau_3=\tau_4$ obtaining $(\sigma,\tau_3) \xrightarrow[]{(write,t)}_{\inc} (\sigma',\tau_4)$. 
\end{proof}

\begin{lemma}
If $(\sigma,\tau_1) \xrightarrow[]{(end,t)}_{\sat} (\sigma',\tau_2)$, $\tau_2 \sqsubseteq \tau_4$, and $\tau_4$ is total then there exists a $\tau_3$ such that $(\sigma,\tau_3) \xrightarrow[]{(end,t)}_{\inc} (\sigma',\tau_4)$ and $\tau_1 \sqsubseteq \tau_3$.
\end{lemma}
\begin{proof}
This follows in the same lines as Lemma \ref{lem:wr}.
\end{proof}

\begin{lemma}
If $(\sigma,\tau_1) \xrightarrow[]{(read,t,t')}_{\sat} (\sigma',\tau_2)$, $\tau_2 \sqsubseteq \tau_4$, and $\tau_4$ is total then there exists a $\tau_3$ such that $(\sigma,\tau_3) \xrightarrow[]{(read,t,,t')}_{\inc} (\sigma',\tau_4)$ and $\tau_1 \sqsubseteq \tau_3$.
\label{lem:read}
\end{lemma}

\begin{proof}
Let $\tau_1= \langle \tran_1,\tpo_1,\trf_1,\tco_1 \rangle$, $\tau_2= \langle \tran_2,\tpo_2,\trf_2,\tco_2 \rangle$, and $\tau_4= \langle \tran_4,\tpo_4,\trf_4, \tco_4 \rangle$. By definition of $\xrightarrow[]{(read,t,t')}_{\sat}$, we have $ev = r(p,t,x,v)$, $\tran_2 = \tran_1$, $\tpo_2 = \tpo_1$, $\trf_2 = \trf_1 \cup t'[\trf] t$, and $ \tco_2 = \tco_1 \cup \tco_2'$, where  $\tco_2' = \tco_1 \cup \{t'' [\tco] t' \mid t'' \in \vbl(\tau_1,t,x)\}$, and, if there exists $t_2$ [$\trf_1$]$^y$ $t$, and $t' \in \tran_1^{w,y}$, then $\tco_2' = \tco_2'  \cup t'$ [$\tco$] $t_2$. Since $\tau_2 \sqsubseteq \tau_4$ it follows that $\tran_4= \tran_2$, $\tpo_4 = \tpo_2$, $\trf_4 = \trf_2$, and $ \tco_2 \subseteq \tco_4$.\\

Define $\tau_3 = \langle \tran_3,\tpo_3,\trf_3,\tco_3 \rangle$ such that $\tran_3 = \tran_1$, $\tpo_3 = \tpo_1$, $\trf_3 = \trf_1 = \trf_4|_{\tran_3}$, $\tco_3 = \tco_4|_{\tran_3}$. 
It follows that $\tau_3 \xrightarrow[]{(read,t,t')}_{\inc} \tau_4$.\\

 We show that $\tco_1 \subseteq \tco_3$. Consider $t_1$ [$\tco_1$] $t_2$. It follows that $t_1$ [$\tco_2$] $t_2$ and hence $t_1$ [$\tco_4$] $t_2$. Since $t_1, t_2 \in \tran_1$ and $\tco_3 = \tco_4|_{\tran_3}$, we obtain  $t_1$ [$\tco_3$] $t_2$.  
\end{proof}

\begin{lemma}
If $(\sigma,\tau_1) \xrightarrow[]{*}_{\sat} (\sigma',\tau_2)$, $\tau_2 \sqsubseteq \tau_4$, and $\tau_4$ is total then there exists a $\tau_3$ such that $(\sigma,\tau_3) \xrightarrow[]{*}_{\inc} (\sigma',\tau_4)$ and $\tau_1 \sqsubseteq \tau_3$.
\label{lem:ex}
\end{lemma}

\begin{proof}
Follows from Lemmas  \ref{lem:begin} to \ref{lem:read}.
\end{proof}

\begin{lemma}
	$\{ weak(\tau) | \tau \in \big[[ \sigma]\big]_{\ccvt}^{\sat} \} \subseteq \{ weak(\tau) | \tau \in \big[[ \sigma]\big]^{\inc}_{\ccvt} \}$ for any configuration $\sigma$.
	\label{lem:one}
\end{lemma}
\begin{proof}
Assume $\tau \in 	\big[[ \sigma]\big]_{\ccvt}^{\sat}$. 
We show that there is a trace $\tau'$ s.t. $\tau' \in 
\big[[ \sigma]\big]_{\ccvt}^{\inc}$ s.t. $\tau \subseteq \tau'$. Then we obtain the result.

Since $\tau \in 	\big[[ \sigma]\big]_{\ccvt}^{\sat}$, we know that 
$(\sigma, \tau_{\emptyset}) \xrightarrow[]{*}_{\sat} (\sigma',\tau)$ for some 
configuration $\sigma'$. That is, there is a sequence  
$(\sigma_0, \tau_0) \xrightarrow[]{}_{\sat} 
(\sigma_1, \tau_1) \xrightarrow[]{}_{\sat}  
(\sigma_2, \tau_2) \xrightarrow[]{}_{\sat} \dots 
 \xrightarrow[]{}_{\sat} (\sigma_n, \tau_n)$ with 
 $\sigma_0=\sigma$, $\tau_0=\tau_{\emptyset}$, 
 $\sigma_n=\sigma'$ and $\tau_n=\tau$. Since $\tau_{\emptyset}$ is a fulfilled trace, and $\tau_{\emptyset} \models \ccvt$, it follows by  
 Lemmas \ref{lem:f1}, \ref{lem:f2}, \ref{lem:f3} and \ref{lem:f4} that 
 $\tau$ is fulfilled and $\tau \models \ccvt$.  By Theorem \ref{ccv-sat}
it follows that $\tau$ is $\ccvt$ consistent, that is, there is a total 
trace $\tau'$ s.t. $\tau \sqsubseteq \tau'$ and $\tau' \models \ccvt$. 
By Lemma \ref{lem:ex}, there is a sequence 
 $(\sigma_0, \tau'_0) \xrightarrow[]{}_{\inc} 
(\sigma_1, \tau'_1) \xrightarrow[]{}_{\inc}  
(\sigma_2, \tau'_2) \xrightarrow[]{}_{\inc} \dots 
 \xrightarrow[]{}_{\inc} (\sigma_n, \tau'_n)$ such that 
 $\tau'_n=\tau'$ and $\tau_{\emptyset} \sqsubseteq \tau'_0$. 
 
 \smallskip 
 
 Note that if we have $\tau_{\emptyset} \sqsubset \tau'_0$, 
 and have the run above in the incremental semantics, then we also have a run
 $(\sigma_0, \tau_{\emptyset})  
 \xrightarrow[]{*}_{\inc} (\sigma_n, \tau'_n)$. This can be seen as follows. 
 If there is no transaction having a write event in the run from $(\sigma_0, \tau'_0)$, then no $\textcolor{orange}{co}$ edges get added in the sequence, so in this case we can assume $\tau'_0=\tau_0$ and 
 $\tau'_n=\tau_n$, and they are total vacuously. If we encounter write transitions in some transactions in the sequence, then, even if we begin with $\tau'_0=\tau_{\emptyset}$,  
 we can make total, the $\textcolor{orange}{co}$ edges whenever write transitions happen, and reach $\tau'_n$.
 Since $\tau'_0$ and $\tau_{\emptyset}$ differ only in the $\textcolor{orange}{co}$ edges, the run starting with $(\sigma_0, \tau_{\emptyset})$ 
 can ``catch up'' with the run starting from $(\sigma_0, \tau'_0)$ and reach $\tau'_n$.

 Thus, we obtain the run  $(\sigma_0, \tau_{\emptyset}) 
 \xrightarrow[]{*}_{\inc} (\sigma_n, \tau')$, and hence, $\tau' \in \big[[ \sigma]\big]_{\ccvt}^{\inc}$. 
   
\end{proof}

From Lemma \ref{lem:sim} and Lemma \ref{lem:one}, we obtain 
\begin{lemma}
$\{ weak(\tau) | \tau \in \big[[ \sigma]\big]_{\ccvt}^{\sat} \} \subseteq \{ weak(\tau) | \tau \in \big[[ \sigma]\big]_{\ccvt} \}$\end{lemma}

\subsection{$\{ weak(\tau) | \tau \in \big[[ \sigma]\big]^{\sat}_{\ccvt} \} \supseteq \{ weak(\tau) | \tau \in \big[[ \sigma]\big]_{\ccvt} \}$}
\label{app:dir2}
\begin{lemma}
	Given $\tau_1= \langle \tran_1,\tpo_1,\trf_1,\tco_1 \rangle$, $\tau_2= \langle \tran_2,\tpo_2,\trf_2,\tco_2 \rangle$, with $(\sigma,\tau_1) \xrightarrow[]{}_{\inc} (\sigma',\tau_2)$ and $\tau_2 \models \ccvt$,   then $\tau_1 \models \ccvt$.
	\label{lem:c1}
\end{lemma}

\begin{proof}
	By definition of $\xrightarrow[]{}_{\inc}$, we know $\tran_1 \subseteq \tran_2$, $\tpo_1 \subseteq \tpo_2$, $\trf_1 \subseteq \trf_2$, and $\tco_1 \subseteq \tco_2$. Since $\tau_2 \models \ccvt$, it follows that 
	 [$\tpo_1 \cup \trf_1 \cup \tco_1$]$^+$ is acyclic and the other two conditions are also true for $\tau_1$. 
	 
\end{proof}

%%%%%%%%

\begin{lemma}
	Given $\tau_1= \langle \tran_1,\tpo_1, \trf_1,\tco_1 \rangle$, $\tau_2= \langle \tran_2,\tpo_2,\trf_2,\tco_2 \rangle$, \\  with $(\sigma,\tau_1) \xrightarrow[]{(read,t,t')}_{\inc} (\sigma',\tau_2)$, reading an event $ev = r(p,t,x,v)$, and 
	$\tau_2 \models \ccvt$, then $t' \in \rbl(\tau_1,t,x)$.
	\label{lem:rdl}
\end{lemma}

\begin{proof}
From the definition of $\xrightarrow[]{(read,t,t')}_{\inc}$, we know $\tran_1 = \tran_2$, $\tpo_2 = \tpo_1$, $\trf_2 = \trf_1 \cup t'[\trf] t$, $\tco_2 \supseteq \tco_1$. $\tau_1$ and $\tau_2$ are total. Assume $t' \notin \rbl(\tau_1,t,x)$. By the definition of readable sets, $t' \notin \rbl(\tau_1,t,x)$ implies ${\tt{cond1}} \vee {\tt{cond2}} \vee {\tt{cond3}}
\vee {\tt{cond4}}$. Using lemmas from section \ref{sec:cyc1},  
we know that ${\tt{cond1}} \vee {\tt{cond2}} \vee {\tt{cond3}}
\vee {\tt{cond4}}$ iff $[\textcolor{red}{po}_2 \cup \textcolor{blue}{rf}_2 \cup \textcolor{orange}{co}_2]^+$ is cyclic, contradicting 
$\tau_2 \models \ccvt$.

\end{proof}

%%%%%%%%%%%%%%%%
\begin{lemma}
If $\tau \sqsubseteq \tau'$ then $\rbl(\tau',t,x) \subseteq \rbl(\tau,t,x)$.
\label{lem:rdl1}
\end{lemma}
\begin{proof}
If $t' \in \rbl(\tau',t,x)$, then by lemmas from 
 section \ref{sec:cyc2}, we know that $\neg {\tt{cond1}} \wedge \neg {\tt{cond2}} \wedge \neg {\tt{cond3}}\wedge \neg {\tt{cond4}}$.   Since each ${\tt{cond}}$ represents a   $[\textcolor{red}{po}_2 \cup \textcolor{blue}{rf}_2 \cup \textcolor{orange}{co}_2]^+$  cycle, and 
$\tau \sqsubseteq \tau'$, the acyclicity of $\tau \sqsubseteq \tau'$ implies 
that of $[\textcolor{red}{po}_1 \cup \textcolor{blue}{rf}_1 \cup \textcolor{orange}{co}_1]^+$. Thus, $\neg {\tt{cond1}} \wedge \neg {\tt{cond2}} \wedge \neg {\tt{cond3}}\wedge \neg {\tt{cond4}}$ also hold good for $\tau$ and hence $t' \in \rbl(\tau,t,x)$.

\end{proof}

%%%%%%%%%%%%
\begin{lemma}
If $(\sigma,\tau_1) \xrightarrow[]{(begin,t)}_{\inc} (\sigma',\tau_2)$, and $\tau_3 \sqsubseteq \tau_1$,  then there exists a $\tau_4$ such that $(\sigma,\tau_3) \xrightarrow[]{(begin,t)}_{\sat} (\sigma',\tau_4)$ and $\tau_4 \sqsubseteq \tau_2$.
\label{lem:c2}
\end{lemma}

\begin{proof}
Let $\tau_1= \langle \tran_1,\tpo_1,\trf_1,\tco_1 \rangle$, $\tau_2= \langle \tran_2,\tpo_2,\trf_2,\tco_2 \rangle$, and $\tau_3 = \langle 
\tran_3,\tpo_3,\trf_3,\tco_3 \rangle$. By definition of $\xrightarrow[]{(begin,t)}_{\inc}$, we have $\tran_2 = \tran_1 \cup \{t\}$, $\tpo_2 = \tpo_1 \cup \{(t',t) \mid t'$ is the last transaction executed before $t$  in some process $p\}$, $\trf_2 = \trf_1$, and $ \tco_2 = \tco_1$, and $\tco_2$ is total. Since $\tau_3 \sqsubseteq \tau_1$ it follows that $\tran_3 = \tran_1$, $\tpo_3 = \tpo_1$, $\trf_3 = \trf_1$, and $ \tco_3 \subseteq \tco_1$.

Define $\tau_4 = \langle \tran_4,\tpo_4,\trf_4,\tco_4 \rangle$ such that $\tran_4 = \tran_3 \cup \{t\}$, $\tpo_4 = \tpo_3 \cup \{(t',t) \mid 
 t'$ is the last transaction executed before $t$  in some process $p\}$, 
 $\trf_4 = \trf_3$, $\tco_4 = \tco_3$. It follows that $\tau_3 \xrightarrow[]{t}_{\sat} \tau_4$. We need to show that $\tco_4 \subseteq \tco_2$. Since $\tco_1 = \tco_2$, $\tco_3 \subseteq \tco_1$ and $\tco_4 = \tco_3$, we get $\tco_4 \subseteq \tco_2$.  
\end{proof}
%%%%%%%%%%%%%%%%%%%
\begin{lemma}
If $(\sigma,\tau_1) \xrightarrow[]{(write,t)}_{\inc} (\sigma',\tau_2)$, and $\tau_3 \sqsubseteq \tau_1$, then there exists a $\tau_4$ such that $(\sigma,\tau_3) \xrightarrow[]{(write,t)}_{\sat} (\sigma',\tau_4)$ and $\tau_4 \sqsubseteq \tau_2$.
\label{lem:c3}
\end{lemma}

\begin{proof}
Let $\tau_1= \langle \tran_1
,\tpo_1,\trf_1,\tco_1 \rangle$, $\tau_2= \langle \tran_2,\tpo_2,\trf_2,\tco_2 \rangle$, and $\tau_3 = \langle \tran_3,\tpo_3,\trf_3,\tco_3 \rangle$. By definition of $\xrightarrow[]{(write,t)}_{\inc}$, we have $\tran_2 = \tran_1$, $\tpo_2 = \tpo_1$, $\trf_2 = \trf_1$, and $ \tco_2 \supseteq \tco_1$, and $\tco_2$ is total. Since $\tau_3 \sqsubseteq \tau_1$ it follows that $\tran_3 = \tran_1$, $\tpo_3 = \tpo_1$, $\trf_3 = \trf_1$, and $ \tco_3 \subseteq \tco_1$.

Define $\tau_4 = \langle \tran_4,\tpo_4,\trf_4,\tco_4 \rangle$ such that $\tran_4 = \tran_3$, $\tpo_4 = \tpo_3$, $\trf_4 = \trf_3$, $\tco_4 = \tco_3$. It follows that $\tau_3 \xrightarrow[]{(write,t)}_{\sat} \tau_4$. Since $\tco_1 \subseteq \tco_2$, $\tco_3 \subseteq \tco_1$ and $\tco_4 = \tco_3$, we get $\tco_4 \subseteq \tco_2$.  
\end{proof}
%%%%%%%%%%%%%%
\begin{lemma}
If $(\sigma,\tau_1) \xrightarrow[]{(end,t)}_{\inc} (\sigma',\tau_2)$, and $\tau_3 \sqsubseteq \tau_1$, then there exists a $\tau_4$ such that $(\sigma,\tau_3) \xrightarrow[]{(end,t)}_{\sat} (\sigma',\tau_4)$ and $\tau_4 \sqsubseteq \tau_2$.
\label{lem:c4}
\end{lemma}
\begin{proof}
The proof follows trivially since $\sigma=\sigma'$ and $\tau_1=\tau_2$.	
Choosing $\tau_3=\tau_1$ and $\tau_4=\tau_2$, we have the result.
\end{proof}

%%%%%%%%%%%%%%
\begin{lemma}
If $(\sigma,\tau_1) \xrightarrow[]{(read,t,t')}_{\inc} (\sigma',\tau_2)$, $\tau_3 \sqsubseteq \tau_1$, and $\tau_2 \models \ccvt$  then there exists a $\tau_4$ such that $(\sigma,\tau_3) \xrightarrow[]{(read,t,t')}_{\sat} (\sigma',\tau_4)$ and $\tau_4 \sqsubseteq \tau_2$.
\label{lem:c5}
\end{lemma}

\begin{proof}
Let $\tau_1= \langle \tran_1,\tpo_1,\trf_1,\tco_1 \rangle$, $\tau_2= \langle \tran_2,\tpo_2,\trf_2,\tco_2 \rangle$, and $\tau_3 = \langle \tran_3,\tpo_3,\trf_3,\tco_3 \rangle$. By definition of $\xrightarrow[]{(read,t,t')}_{\inc}$, we have a read event $ev = r(p,t,x,v)$. 
Also,  $\tran_2 = \tran_1$, $\tpo_2 = \tpo_1$, $\trf_2 = \trf_1 \cup t'[\trf] t$, $ \tco_2 \supseteq \tco_1$, and $\tau_2$ is total. Since $\tau_3 \sqsubseteq \tau_1$ it follows that $\tran_3 = \tran_1$, $\tpo_3 = \tpo_1$, $\trf_3 = \trf_1$, and $ \tco_3 \subseteq \tco_1$.

Define $\tau_4 = \langle \tran_4,\tpo_4,\trf_4,\tco_4 \rangle$ such that $\tran_4 = \tran_3$, $\tpo_4 = \tpo_3$, $\trf_4 = \trf_3 \cup t'[\trf] t$, $\tco_4 = \tco_3 \cup \tco_3'$, where  $\tco_3' = \tco_3 \cup \{t'' [\tco] t' \mid t'' \in \vbl(\tau_3,t,x)\}$, and if $\exists t_2$ [$\trf_1$]$^y$ $t$, and $t' \in \tran^{w,y}$, then $\tco_3' = \tco_3' \cup t'$ [$\tco$] $t_2$. From Lemmas \ref{lem:rdl}, \ref{lem:rdl1}
 it follows that $t' \in \rbl(\tau_3,t,x)$, since 
  $t' \in \rbl(\tau_1,t,x)$ and $\tau_3 \sqsubseteq \tau_1$.
 Hence we have $\tau_3 \xrightarrow[]{(read,t,t')}_{\inc} \tau_4$. We need to show that $\tco_4 \subseteq \tco_2$. Assume $t_1 \tco_4 t_2$. We consider the following cases:
\begin{itemize}
	\item[$\bullet$] $t_1 \tco_3 t_2$. Since $\tco_3 \subseteq \tco_1$, it follows that $t_1 \tco_1 t_2$. It follows that $t_1 \tco_2 t_2$.
	\item[$\bullet$] $t_2 = t'$ and $t_1 \in \vbl(\tau_3,t,x)$. Since $t_1 \in \vbl(\tau_3,t,x)$, we have $t_1 [\tpo_3 \cup \trf_3]^+ t$, and hence $t_1 [\tpo_1 \cup \trf_1]^+ t$. It follows that $t_1 [\tpo_2 \cup \trf_2]^+ t$. Since  $\tau_2 \models \ccvt$ and $t' [\trf_2^x] t$, we get $t_1 [\tco_2] t'$.
	\item[$\bullet$] $t_1 = t'$ and $t_2 [\trf_3^y] t$ and $t' \in \tran^{w,y}$. Since $\tau_3 \subseteq \tau_1$ and $(\sigma,\tau_1) \xrightarrow[]{(read,t,t')}_{\inc} (\sigma',\tau_2)$, it follows that $t_2 [\trf_1^y] t$ and $t_2 [\trf_2^y] t$. Since $t_2 [\trf_2^y] t$, and $t$ reads from $t'$ (hence $t' [\tpo_2 \cup \trf_2]^+ t$), and $\tau_2 \models \ccvt$, we get $t' [\tco_2] t_2$, i.e. $t_1 [\tco_2] t_2$.
\end{itemize}
\end{proof}

%%%%%%%%%%%%%%
%\begin{lemma}
%If $\tau_1 \xrightarrow[]{*}_{\inc} \tau_2$, and $\tau_3 \sqsubseteq \tau_1$, then there exists a $\tau_4$ such that $\tau_3 \xrightarrow[]{*}_{\sat} \tau_4$ and $\tau_4 \sqsubseteq \tau_2$.
%\end{lemma}
%
%\begin{proof}
%Follows from Lemma 19-22.
%\end{proof}

\begin{lemma}
$\{ weak(\tau) | \tau \in \big[[\sigma]\big]_{\ccvt}^{\inc} \} \subseteq \{ weak(\tau) | \tau \in \big[[ \sigma]\big]_{\ccvt}^{\sat} \}$ for any configuration $\sigma$.
\label{lem:c6}
\end{lemma}
\begin{proof}
Suppose $\tau \in \big[[\sigma]\big]_{\ccvt}^{\inc}$. We show that there is a trace $\tau' \in \big[[ \sigma]\big]_{\ccvt}^{\sat}$ s.t. $\tau' \sqsubseteq \tau$. Then the result follows immediately. 

Since $\tau \in  \big[[\sigma]\big]_{\ccvt}^{\inc}$, it follows that $\tau \models \ccvt$ and that $(\sigma, \tau_{\emptyset}) \xrightarrow[]{*}_{\inc} (\sigma', \tau)$ for some configuration $\sigma'$. That is, there is a sequence   $(\sigma_0, \tau_0 \xrightarrow[]{}_{\inc} (\sigma_1, \tau_1) \xrightarrow[]{}_{\inc} \dots \xrightarrow[]{}_{\inc} (\sigma_n, \tau_n)$ where $\sigma_0=\sigma, \tau_0=\tau_{\emptyset}, \sigma_n=\sigma, \tau_n=\tau$.  By Lemma \ref{lem:c1}, we know that $\tau_i \models \ccvt$ 
for all $1 \leq i \leq n$. By Lemmas \ref{lem:c2}, \ref{lem:c3}, \ref{lem:c4}, \ref{lem:c5}, it follows that there is a sequence 
 $(\sigma_0, \tau'_0) \xrightarrow[]{}_{\sat} (\sigma_1, \tau'_1) \xrightarrow[]{}_{\sat} \dots \xrightarrow[]{}_{\sat} (\sigma_n, \tau'_n)$ with 
 $\tau'_0=\tau_{\emptyset}$ and $\tau'_i \sqsubseteq \tau_i$ for 
 $1 \leq i \leq n$. Define $\tau'=\tau'_n$.

\end{proof}

From Lemma \ref{lem:sim} and Lemma \ref{lem:c6} we obtain 
\begin{lemma}
	$\{ weak(\tau) | \tau \in \big[[ \sigma]\big]^{\sat}_{\ccvt} \} \supseteq \{ weak(\tau) | \tau \in \big[[ \sigma]\big]_{\ccvt} \}$. 
\end{lemma}
%%%%%%%%%%%%%%%%%%%%%%%%%%%%%%%%%%%%%%%%%%%%%%%%%%%
\section{Completeness}
\label{app:complete-ccv}
In this section, we show the completeness of the DPOR algorithm. More precisely, for any configuration $\sigma$, terminating run $\rho \in \exec(\sigma)$ and total trace $\tau$ s.t. $\tau \models \rho$, 
we show that $ExploreTraces(\sigma, \tau_{\emptyset}, \epsilon)$ will produce a recursive visit $ExploreTraces(\sigma', \tau', \pi)$ for some terminal $\sigma'$, $\tau'$, and $\pi$ where $weak(\tau')=weak(\tau)$.   First we give some definitions and auxiliary lemmas.

Let  $\pi = \alpha_{t_1} \alpha_{t_2} \dots \alpha_{t_n}$ be an observation sequence where  $\alpha_t = \beginact(p,t) \dots$ \plog{end}$(p,t)$.
 $\alpha_t$ is called an \emph{observable}, and is a sequence 
 of events from transaction $t$.  
Given $\pi$, a configuration $\sigma$, and a trace $\tau$, we define 
$\langle \sigma,\tau \rangle \vdash_{\tt{G}} \pi$ to represent a sequence 
$\langle \sigma_0 , \tau_0 \rangle \xrightarrow[]{\alpha_{t_1}}_{\sat} 
\langle \sigma_1,\tau_1 \rangle \xrightarrow[]{\alpha_{t_2}}_{\sat} \cdot \cdot \cdot \xrightarrow[]{\alpha_{t_n}}_{\sat} \langle \sigma_n,\tau_n \rangle$, where 
$\sigma_0 = \sigma$, $\tau_0 = \tau$ and 
$\pi = \alpha_{t_1} \alpha_{t_2} \dots \alpha_{t_n}$. Moreover, we define $\pi (\sigma,\tau) := \langle \sigma_n,\tau_n \rangle$. We define $\tau \vdash_{\tt{G}} \pi$ in similar manner, when there exists some $\sigma$ 
s.t.  $(\sigma, \tau) \vdash_{\tt{G}} \pi$.

 $\langle \sigma, \tau \rangle$ is $terminal$ if $\sigma$ is terminal. We define $\langle \sigma,\tau \rangle \vdash_{\tt{G_T}} \pi$ to say that $(i)$ $ \langle \sigma,\tau \rangle \vdash_{\tt{G}} \pi$ and $(ii)$ $\pi(\sigma,\tau)$ is terminal.

\begin{definition}($p$-free and $t$-free observation sequences)
For a process  $p \in \mathbf{P}$, we say that an observation sequence $\pi$ is $p$-free if   all observables $\alpha_{t}$ in $\pi$ pertain to 
transactions $t$ not in $p$. 
For a transaction $t$ issued in $p$ we say that $\pi$ is $t$-free if $\pi$ is $p$-free. 
\end{definition}

\begin{definition}(Independent Observables)
For observables $\alpha_{t_1}$ and $\alpha_{t_2}$, we write $\alpha_{t_1} \sim  \alpha_{t_2}$ to represent they are independent. 
This means 
$(i)$ $t_1,t_2$ are transactions issued in different processes, that is, 
 $t_1$ is issed in $p_1$, $t_2$ is issued  in $p_2$, with $p_1 \neq p_2$,  
$(ii)$ no read event $r(p_2,t_2,x,v)$ of transaction $t_2$ reads from $t_1$, and 
$(iii)$ no read event $r(p_1,t_1,x,v)$ of transaction $t_1$ reads from $t_2$.	
Thus, $\neg(\alpha_{t_1} \sim  \alpha_{t_2})$ if either $t_1, t_2$ are issued in the same process, or there is a $\trf$ relation between $t_1, t_2$. That is, $\neg(\alpha_{t_1} \sim  \alpha_{t_2})$ iff $t_1 [\tpo \cup \trf]^+ t_2$ or  $t_2 [\tpo \cup \trf]^+ t_1$.

\end{definition}
 
 \begin{definition}(Independent Observation Sequences)
Observation sequences $\pi^1, \pi^2$ are called independent written $\pi^1 \sim \pi^2$ if there are observables $\alpha_{t_1}$, $\alpha_{t_2}$, and observation sequences $\pi'$ 
and $\pi''$ such that $\pi^1 = \pi' \cdot \alpha_{t_1} \cdot \alpha_{t_2} \cdot \pi''$, 
$\pi^2 = \pi' \cdot \alpha_{t_2} \cdot \alpha_{t_1} \cdot \pi''$, 
and $\alpha_{t_1} \sim \alpha_{t_2}$. 
In other words, we get $\pi^2$ from $\pi^1$ by swapping neighbouring independent observables corresponding to transactions $t_1$ and $t_2$. 
\end{definition}
We use $\approx$ to denote reflexive transitive closure of $\sim$.

\begin{definition}(Equivalent Traces)
For traces $\tau_1 = \langle \tran_1, \textcolor{red}{po}_1, \textcolor{blue}{rf}_1, \textcolor{orange}{co}_1 \rangle$ and $\tau_2 = \langle \tran_2, \textcolor{red}{po}_2, \textcolor{blue}{rf}_2, \textcolor{orange}{co}_2 \rangle$, we say $\tau_1, \tau_2$ are equivalent denoted $\tau_1 \equiv \tau_2$ if $\tran_1 = \tran_2$, $\tpo_1 = \tpo_2$, $\trf_1 = \trf_2$ and for all $t_1$,$t_2 \in \tran_1^{w,x}$ for all variables $x$, we have $t_1$ [$\tpo_1 \cup \trf_1 \cup \tco_1^x$] $t_2$ iff $t_1$ [$\tpo_2 \cup \trf_2 \cup \tco_2^x$] $t_2$.
	
\end{definition}

%%%%%%%%
\begin{lemma}
$((\tau_1 \equiv \tau_2) \wedge \tau_1 \vdash_{\tt{G}} \alpha_t) \Rightarrow (\tau_2 \vdash_{\tt{G}} \alpha_t \wedge (\alpha_t(\tau_1) \equiv \alpha_t(\tau_2)))$.
\label{lemma g-1}
\end{lemma}
\begin{proof}
Assume 	$\tau_1 \vdash_{\tt{G}} \alpha_t$ for an observable $\alpha_t$, and 
$\tau_1=(\tran_1, \tpo_1, \trf_1, \tco_1)$, 
$\tau_2=(\tran_2, \tpo_2, \trf_2, \tco_2)$ with $\tau_1 \equiv \tau_2$. Then we know that $\tran_1=\tran_2, \tpo_1=\tpo_2, \trf_2=\trf_1$. 
 
 Since $\tau_1 \vdash_{\tt{G}} \alpha_t$, let  $\tau_1 \xrightarrow[]{\alpha_t}_{\sat} \tau'$. 
 $\tau'=(\tran', \tpo', \trf', \tco')$ where $\tran'=\tran_1 \cup \{t\}$, 
 $\tpo'=\tpo_1 \cup \{(t_1,t) \mid t_1 \in \tran_1$ is in the same process as $t\}$,  $\tco_1 \subseteq \tco'$ 
 and $\trf_1 \subseteq \trf'$. $\tco'$ can contain $(t',t)$ for some 
 $t' \in \tran_1$, when $t',t \in {\tran'}^{w,x}$ for some variable $x$, based 
 on the fulfilled semantics. In particular if we have 
 $t_1 {\trf'}^x t_2$ and $t_3 (\trf'\cup  \tpo' \cup {\tco'}^x)^+ t_2$, then    
 $t_3 {\tco'}^x t_1$.

 Since $\tau_1 \equiv \tau_2$, for any transactions $t', t'' $ in $\tran_1=\tran_2$, $t' [\tpo_1 \cup \tco_1^x \cup \trf_1] t''$ iff $t' [\tpo_2 \cup \tco_2^x \cup \trf_2] t''$ for all variables $x$. In particular, $t' \tco_1^x t''$ iff $t' \tco_2^x t''$ for all $x$. 
 Now, let us construct a trace $\tau''=(\tran', \tpo', \trf', \tco'')$,
 where $\tco''$ is the smallest set such that $\tco_2 \subseteq \tco''$ and 
  whenever $t_1 {\trf'}^x t_2$ and $t_3 (\trf'\cup  \tpo' \cup {\tco''}^x)^+ t_2$, then $t_3 {\tco''}^x t_1$.

   Since $t' [\tpo_1 \cup \trf_1 \cup \tco_1^x] t''$ iff $t' [\tpo_2 \cup \trf_2 \cup \tco_2^x] t''$ for all $x$, and all $t', t'' \in \tran_1=\tran_2$, and $\tco''$ is the smallest extension of $\tco_2$  based 
   on the fulfilled semantics, along with the fact that 
   $\tpo'=\tpo'', \trf'=\trf''$, we obtain for any two 
   transactions $t_1, t_2 \in \tran'=\tran''$, 
   $t_1 [\tpo' \cup \trf' \cup \tco'] t_2$ iff  $t_1 [\tpo'' \cup \trf''
   \cup \tco''] t_2$. This gives $\tau' \equiv \tau''$. 
    
      This also gives $\tau_2 \xrightarrow[]{\alpha_t}_{\sat} \tau''$,
  that is, $\tau_2 \vdash_{\tt{G}} \alpha_t$  and indeed $\alpha_t(\tau_1)=\tau' \equiv \tau''=\alpha_t(\tau_2)$.

\end{proof}

%%%%%%%%%%
\begin{lemma}
If $\tau \vdash_{\tt{G}} \alpha_{t_1} \cdot \alpha_{t_2}$ and $\alpha_{t_1} {\sim} \alpha_{t_2}$ then $\tau \vdash_{\tt{G}} \alpha_{t_2} {\cdot} \alpha_{t_1}$ and $(\alpha_{t_1} {\cdot} \alpha_{t_2})(\tau) \equiv (\alpha_{t_2}{ \cdot} \alpha_{t_1})(\tau)$.
\label{lemma g-2}
\end{lemma}
\begin{proof}
Let $\tau = \langle \tran , \tpo, \trf,\tco \rangle$ be a trace and let $t_1$ be a transaction issued in process $p_1$, and $t_2$ be a transaction issued in process $p_2$, with $p_1 \neq p_2$. Assume $\tau \vdash_{\tt{G}} \alpha_{t_1} \cdot \alpha_{t_2}$, with $\alpha_{t_1} {\sim} \alpha_{t_2}$. 

%\subsection*{Proving $\tau \vdash_{\tt{G}} \alpha_{t_2} {\cdot} \alpha_{t_1}$}

We consider the following cases.
\begin{itemize}
    \item [$\bullet$] $t_1,t_2 \notin \tran^r$. In this case $\tau \vdash_{\tt{G}} \alpha_{t_2} \cdot \alpha_{t_1}$ holds trivially.
    
     $(\alpha_{t_1} \cdot \alpha_{t_2})(\tau) = (\alpha_{t_2} \cdot \alpha_{t_1})(\tau) = \langle \tran' , \tpo' , \trf, \tco \rangle$, where $\tran' = \tran \cup \{t_1,t_2\}$ and $\tpo' = \tpo \cup \{ (t,t_1) | t \in p_1\} \cup \{(t',t_2) | t' \in p_2 \}$.
    \item [$\bullet$] $t_1 \in \tran^w$, $t_1 \notin \tran^r$ and $t_2 \in \tran^r \cap \tran^w$. 
    Let $\tau_1 = \alpha_{t_1}(\tau)$. 
    We know that $\tau_1 = \langle \tran_1 , \tpo_1 , \trf_1,\tco_1 \rangle$, where 
    $\tran_1 = \tran \cup \{ t_1 \}$, and $\tpo_1 = \tpo \cup \{ (t,t_1) | t \in p_1\}$, with $\trf_1 = \trf$ since there are no read events in $t_1$, and $\tco_1 = \tco$ since by the fulfilled semantics, when $ \trf$ remain same, there are no $\tco$ edges to be added.
    
    Consider $\tau_2 = \alpha_{t_2}(\tau_1) = \langle \tran_2, \tpo_2, \trf_2, \tco_2 \rangle$. 
    Since $t_2 \in \tran^r$, we know that $t_2$ has read events.
    \smallskip

    Let there be $n$ read events $ev_1 \dots ev_n$ in transaction $t_2$, 
    reading from transactions $t'_1, \dots, t'_n$ on variables $x_1, \dots, x_n$.  
    Hence we get a sequence $\tau_1 \xrightarrow[]{(begin,t_2)}_{\sat} \dots \tau'_{i_1} \xrightarrow[]{(read,t_2,t'_1)}_{\sat}  \tau_{i_1}  \xrightarrow[]{}_{\sat}\dots  
    %\xrightarrow[]{}_{\sat} \dots \tau'_{i_2} \xrightarrow[]{(ev_2,t'_2)}_{\sat} \tau_{i_2} \xrightarrow[]{}_{\sat} \dots 
    \tau'_{i_n} \xrightarrow[]{(read,t_2,t'_n)}_{\sat} \tau_{i_n} \dots \xrightarrow[]{(end,t_2)}_{\sat} \tau_2$.
    Hence $\tran_2 = \tran_1 \cup \{t_2\}$, $\tpo_2 = \tpo_1 \cup \{(t',t_2) | t' \in p_2\}$, $\trf_2 = \trf_1 \cup (\trf_{i_1} \cup \trf_{i_2} \dots \cup \trf_{i_n})$, and $\tco_2 = \tco_1 \cup (\tco_{i_1} \cup \tco_{i_2} \dots \cup \tco_{i_n})$.
    Since $\tau_1 \vdash_{\tt{G}} \alpha_{t_2}$,  for all $ev_i : 1 \le i \le n$, we have $t'_i \in \rbl(\tau_1,t_2,x_i)$.
    
    Since $\alpha_{t_1} \sim \alpha_{t_2}$, we know that for all $ev_i : 1 \le i \le n$, we have $t'_i \in \rbl(\tau,t_2,x_i)$. It follows that $\tau \vdash_{\tt{G}} \alpha_{t_2}$.
    Define $\tau_3 = \langle \tran_3, \tpo_3, \trf_2, \tco_2 \rangle$, where $
    \tran_3 = \tran \cup \{t_2\}$ and $\tpo_3 = \tpo \cup \{(t',t_2) | t' \in p_2\}$. It follows that $\alpha_{t_2}(\tau) = \tau_3$, $\tau_3 \vdash_{\tt{G}} \alpha_{t_1}$ and $\tau_2 = \alpha_{t_1}(\tau_3) = \alpha_{t_2}(\alpha_{t_1}(\tau))$.
    \item [$\bullet$] $t_2 \in \tran^w$ and $t_1 \in \tran^r \cap \tran^w$. Similar to previous case.
    \item [$\bullet$] $t_1, t_2 \in \tran^r \cap \tran^w$. 
    Let $\tau_1 = \alpha_{t_1}(\tau) = \langle \tran_1, \tpo_1, \trf_1, \tco_1 \rangle$ and $\tau_2 = \alpha_{t_2}(\tau_1)$. Since $t_1 \in \tran^r$, we know that $t_1$ has read events. 
    Let there be $n$ read events $ev_1 \dots ev_n$ in transaction $t_1$, reading from transactions $t'_1, \dots, t'_n$ on variables 
    $x_1, \dots, x_n$. 
    Hence we get the sequence $\tau \xrightarrow[]{(begin,t_1)}_{\sat} \dots \tau'_{i_1} \xrightarrow[]{(read,t_1,t'_1)}_{\sat}  \tau_{i_1} \xrightarrow[]{}_{\sat}\dots  
    %\xrightarrow[]{}_{\sat} \dots \tau'_{i_2} \xrightarrow[]{(ev_2,t'_2)}_{\sat} \tau_{i_2} \xrightarrow[]{}_{\sat} \dots 
    \tau'_{i_n} \xrightarrow[]{(read,t_1,t'_n)}_{\sat} \tau_{i_n} \dots \xrightarrow[]{(end,t_1)}_{\sat} \tau_1$.
    Since $t_2 \in \tran^r$, we know that $t_2$ has read events. 
    Let there be  $m$ read events $ev'_1 \dots ev'_m$ in transaction $t_2$, reading from transactions $t''_1, \dots, t''_m$ on variables 
    $y_1, \dots, y_m$.  
    Then we get the sequence $\tau_1 \xrightarrow[]{(begin,t_2)}_{\sat} \dots \tau'_{j_1} \xrightarrow[]{(read,t_2,t''_1)}_{\sat}  \tau_{j_1}  \xrightarrow[]{}_{\sat} \dots 
    %\tau'_{j_2} \xrightarrow[]{(ev'_2,t''_2)}_{\sat} \tau_{j_2} \xrightarrow[]{}_{\sat} \dots 
    \tau'_{j_n} \xrightarrow[]{(read,t_2,t''_m)}_{\sat} \tau_{j_n} \dots \xrightarrow[]{(end,t_2)}_{\sat} \tau_2$. 
    
    $\mathbf{Proving}$ $\mathtt{ \tau \vdash_{\tt{G}} \alpha_{t_2} {\cdot} \alpha_{t_1}}$
    
    Since $\tau_1 = \alpha_{t_1}(\tau)$, for all read events $ev_i$ such that $ev_i.trans = t_1$, we have $t'_i \in \rbl(\tau,t_1,x_i)$.
    Since $\tau_2 = \alpha_{t_2}(\tau_1)$, for all read events $ev'_j$ such that $ev'_j.trans = t_2$, we have $t''_j \in \rbl(\tau_1,t_2,y_j)$. 
    Since $\alpha_{t_1} \sim \alpha_{t_2}$, 
    it follows that, we have $t''_j \in \rbl(\tau,t_2,y_j)$ for all read events $ev'_j$ such that $ev'_j.trans = t_2$. Hence $\tau \vdash_{\tt{G}} \alpha_{t_2}$. 
    \smallskip

    Consider $\tau_3 = \alpha_{t_2}(\tau) = \langle \tran_3, \tpo_3, \trf_3, \tco_3 \rangle $. To show that $\tau \vdash_{\tt{G}} \alpha_{t_2} \alpha_{t_1}$, 
    we show that for all read events $ev_i$ such that $ev_i.trans = t_1$,  $t'_i \in \rbl(\tau_3,t_1,x_i)$. We prove this using contradiction.
     Assume that $\exists t'_i$ s.t. $t'_i \notin \rbl(\tau_3,t_1,x_i)$.

    \medskip 
    \smallskip

    If $t'_i \notin \rbl(\tau_3,t_1,x_i)$, then 
    there is a $t'_k$ such that (i) $t'_k \in \vbl(\tau_3,t_1,x_i)$ and (ii) $t'_i [\tpo_3 \cup \trf_3 \cup \tco_3]^+ t'_k$.
     
     \medskip 
     \smallskip

       If   (i) is true, that is, $t'_k \in \vbl(\tau_3,t_1,x_i)$, since $\alpha_{t_1} \sim \alpha_{t_2}$, we also have $t'_k \in \vbl(\tau,t_1,x_i)$. 
        This, combined with $t'_i \in \rbl(\tau,t_1,x_i)$, gives according to the fulfilled semantics, $t'_k [\tco_1] t'_i$.  Going back to (ii), 
    we can have $t'_i [\tpo_3 \cup \trf_3 \cup \tco_3]^+ t'_k$ only if we observed one of the following:
    \begin{itemize}
        \item [(a)] There is a path from $t'_i$ to $t'_k$ in $\tau$; that is, 
        $t'_i [\tpo \cup \trf \cup \tco]^+ t'_k$. This implies that $t'_i \notin \rbl(\tau,t_1,x_i)$ which is a contradiction.
        \item [(b)] There is no direct path from $t'_i$ to $t'_k$, however, 
        there are  transactions  $t''_j,t''_l$ such that, in $\tau$ we had  
        $ t''_j [\tpo \cup \trf \cup \tco]^* t'_k$ and $t'_i [\tpo \cup \trf \cup \tco]^* t''_l$, along with $t''_j \in \rbl(\tau,t_2,y_j)$,  $t''_l \in \vbl(\tau,t_2,y_j)$. Let  $ev'_j = r(p_2,t_2,y_j,v)$ be the read event which reads from $t''_j$, justifying 
        $t''_j \in \rbl(\tau,t_2,y_j)$. 
        
        \smallskip
                Since $t''_j [\tpo \cup \trf \cup \tco]^* t'_k$ and $t'_i [\tpo \cup \trf \cup \tco]^* t''_l$ it follows that $ t''_j [\tpo_1 \cup \trf_1 \cup \tco_1]^* t'_k$, $t'_i [\tpo_1 \cup \trf_1 \cup \tco_1]^* t''_l$. By our assumption, we have $t'_i \in \rbl(\tau,t_1,x_i)$ and $t'_k \in \vbl(\tau,t_1,x_i)$, which  gives us  $t'_k [\tco_1^{x_i}] t'_i$ (already observed in the para before (i)). 
                
                Thus we get  $t''_j [\tpo_1 \cup \trf_1 \cup \tco_1]^*
                t'_k [\tco_1^{x_i}] t'_i [\tpo_1 \cup \trf_1 \cup \tco_1]^*
                 t''_l$, which gives  $t''_j [\tpo_1 \cup \trf_1 \cup \tco_1]^+ t''_l$. Hence $t''_j \notin \rbl(\tau_1,t_2,y_j)$, a  contradiction.
%        \item [(c)] Similar to (b), consider transactions $t''_j,t''_l$ such that $ t''_j [\tpo \cup \trf \cup \tco]^* t'_k$ and $t'_i [\tpo \cup \trf \cup \tco]^* t''_l$, with  $t''_j \in \rbl(\tau,t_2,y_j)$, $t''_l \in \rbl(\tau,t_2,y_j)$, and $t''_l \in \tran^{w,{x_l}}$. Let $t_2$ have read events $ev''_j = r(p_2,t_2,y_j,v_j)$, $ev''_l = r(p_2,t_2,x_l,v_l)$, in the same order, which read from $t''_j$ and $t''_l$ respectively.
%        Since $ t''_j [\tpo \cup \trf \cup \tco]^* t'_k$ and $t'_i [\tpo \cup \trf \cup \tco]^* t''_l$ it follows that $ t''_j [\tpo_1 \cup \trf_1 \cup \tco_1]^* t'_k$, $t'_i [\tpo_1 \cup \trf_1 \cup \tco_1]^* t''_l$. As seen above in case (b), we have $t'_k [\tco_1^{x_i}] t'_i$. In other words we get $t''_j [\tpo_1 \cup \trf_1 \cup \tco_1]^+ t''_l$. Hence $t''_j \notin \rbl(\tau_1,t_2,y_j)$, a contradiction.
    \end{itemize}
    Thus, we have $\neg(t'_i [\tpo_3 \cup \trf_3 \cup \tco_3]^+ t'_k)$. This, for all $1 \leq i \leq n$, $t'_i \in \rbl(\tau_3,t_1,x_i)$. Thus, we now have $\tau \vdash_{\tt{G}} \alpha_{t_2} \alpha_{t_1}$. 
    It remains to show that $(\alpha_{t_1} {\cdot} \alpha_{t_2})(\tau) \equiv (\alpha_{t_2}{ \cdot} \alpha_{t_1})(\tau)$. 
    
    %\subsection*{Proving $(\alpha_{t_1} {\cdot} \alpha_{t_2})(\tau) \equiv (\alpha_{t_2}{ \cdot} \alpha_{t_1})(\tau)$}
    $\mathbf{Proving}$ $\mathtt{(\alpha_{t_1} {\cdot} \alpha_{t_2})(\tau) \equiv (\alpha_{t_2}{ \cdot} \alpha_{t_1})(\tau)}$
    
    Define $\tau_4 {=} \alpha_{t_1}(\tau_3) {=} \alpha_{t_1}.\alpha_{t_2}(\tau){=}
         \langle \tran_4, \tpo_4, \trf_4 , \tco_4 \rangle$. Recall that 
    $\tau_2{=}$$\alpha_{t_2}.\alpha_{t_1}(\tau)$ =$
      \langle \tran_2,\tpo_2, \trf_2, \tco_2 \rangle$.
    \smallskip

    To show that $(\alpha_{t_1} \cdot \alpha_{t_2})(\tau) \equiv (\alpha_{t_2} \cdot \alpha_{t_1})(\tau)$, we show that $\tran_2=\tran_4, \tpo_2=\tpo_4, \trf_2=\trf_4$, and, for any two transactions 
    $t'_k, t'_i \in \tran_2=\tran_4$,    $t'_k [\tpo_2 \cup \trf_2 \cup \tco_2]^+ t'_i$ iff 
    $t'_k [\tpo_4 \cup \trf_4 \cup \tco_4]^+ t'_i$. Of these, trivially, 
    $\tran_2=\tran_4, \tpo_2=\tpo_4$ follow. Since $\alpha_{t_2} \sim \alpha_{t_1}$, we have $\trf_2=\trf_4$. It remains to prove the last condition. 
    
    \medskip 
    
   Assume that $t'_i [\trf^{x_i}_1] t_1 \wedge t'_k \in \vbl(\tau_1,t_1,x_i)$, 
   where $\tau_1=\alpha_{t_1}(\tau)$. Then we have 
   $t'_i [\trf^{x_i}_1] t_1 \wedge t'_k \in \vbl(\tau,t_1,x_i)$, and by the fulfilled semantics, we have $t'_k [\tco_1] t'_i$, and hence 
   $t'_k [\tco_2] t'_i$.  To obtain $\tau_4$, we execute $t_2$ first obtaining $\tau_3$ from $\tau$, and then $t_1$. We show that $t'_k [\tpo_4 \cup \trf_4 \cup \tco_4]^+ t'_i$, proving $t'_k [\tpo_2 \cup \trf_2 \cup \tco_2]^+ t'_i \Rightarrow
    t'_k [\tpo_4 \cup \trf_4 \cup \tco_4]^+ t'_i$.

    \smallskip 
    
     If we have $t'_k \in \vbl(\tau_3,t_1, x_i)$, then we are done since we  have $t'_i \in \rbl(\tau,t_1,x_i)$, hence 
          $t'_i \in \rbl(\tau_3,t_1,x_i)$, thereby obtaining 
          $t'_k \tco_3 t'_i$, and hence $t'_k \tco_4 t'_i$.    
          
          \smallskip 
          
           Assume $t'_k \notin \vbl(\tau_3,t_1, x_i)$.   
   Assume that on executing $t_2$ from $\tau$, we have $t''_l \in \vbl(\tau, t_2, y_j)$, and let $t''_j [\trf^{y_j}_3] t_2$.      
     Then by the fulfilled semantics,   $t''_l [\tco_3] t''_j$ is a new edge which gets added.  
         When we execute $t_1$ next, assume  $t''_m \in \vbl(\tau_3,t_1,x_i)$.   
         Since we have $t'_i \in \rbl(\tau_3,t_1,x_i)$, we obtain $t''_m \tco_4 t'_i$.

     \medskip 
     By assumption, $t'_k \neq t''_m$. However, $t'_k \in \vbl(\tau,t_1,x_i)$. \\
     $t'_k \notin  \vbl(\tau_3,t_1,x_i)$ points to some transaction that 
     blocked the visibility of $t'_k$ in $\tau_3$, by happening after $t'_k$, and which is in $\vbl(\tau_3,t_1,x_i)$.  
     
     \begin{enumerate}
     	\item This blocking transaction could be $t''_m$. If this is the case, we have $t'_k [\tpo_3 \cup \trf_3 \cup \tco_3]^+ t''_m [\tco_4] t'_i$, and hence  $t'_k [\tpo_4 \cup \trf_4 \cup \tco_4]^+ t''_m [\tco_4] t'_i$. 
     	\item The other possibility is that we have  $t''_j$
     	happens before $t''_m$, and $t''_l$ happens after $t'_k$ blocking 
     	$t'_k$ from being in $\vbl(\tau_3,t_1,x_i)$. That is,
     	     $t'_k [\tpo \cup \trf \cup \tco]^* t''_l$ and 
     	     $t''_j [\tpo_4 \cup \trf_4 \cup \tco_4]^* t''_m$.   
         Then we obtain $t'_k [\tpo_4 \cup \trf_4 \cup \tco_4]^* t''_l [\tco^{x_j}_4] t''_j [\tpo_4 \cup \trf_4 \cup \tco_4]^* t''_m [\tco_4] t'_i$. 
     
     \end{enumerate}
        
     Thus, we obtain $t'_k [\tpo_4 \cup \trf_4 \cup \tco_4]^+ t'_i$ as desired.

\end{itemize}
 The converse direction, that is, whenever $t'_k [\tpo_4 \cup \trf_4 \cup \tco_4]^+ t'_i$, we also have $t'_k [\tpo_2 \cup \trf_2 \cup \tco_2]^+ t'_i$ is proved on similar lines. 
    
\end{proof}
%%%%%%%%%%%%
\begin{lemma}
If $\tau_1 \equiv \tau_2$, $\alpha_{t_1} \sim \alpha_{t_2}$, and $\tau_1 \vdash_{\tt{G}} (\alpha_{t_1} \cdot \alpha_{t_2})$,  then (i) $\tau_2 \vdash_{\tt{G}} (\alpha_{t_2} \cdot \alpha_{t_1})$ and (ii) $(\alpha_{t_1} \cdot \alpha_{t_2})(\tau_1) \equiv (\alpha_{t_2} \cdot \alpha_{t_1})(\tau_2)$.
\label{lemma g-3}
\end{lemma}
\begin{proof}
Follows from Lemma \ref{lemma g-1} and Lemma \ref{lemma g-2}.
\end{proof}

From Lemma \ref{lemma g-3}, we get following lemma.
%%%%%%%%
\begin{lemma}
If $\tau_1 \equiv \tau_2$, $\pi_{\tt{T^1}} \sim \pi_{\tt{T^2}}$, and $\tau_1 \vdash_{\tt{G}} \pi_{\tt{T^1}}$ then $\tau_2 \vdash_{\tt{G}} \pi_{\tt{T^2}}$ and $\pi_{\tt{T^1}}(\tau_1) \equiv \pi_{\tt{T^2}}(\tau_2)$.
\label{lemma g-4}
\end{lemma}
%%%%%%%%
 
\begin{lemma}
If $\langle \sigma,\tau \rangle \vdash_{\tt{G_T}} \pi_{\tt{T}}$, $\langle \sigma,\tau \rangle \vdash_{\tt{G}} \alpha_t$ then $\pi_{\tt{T}} = \pi_{\tt{T^1}} \cdot \alpha_t \cdot \pi_{\tt{T^2}}$ for some $\pi_{\tt{T^1}}$ and $\pi_{\tt{T^2}}$ where $\pi_{\tt{T^1}}$ is $t$-free.
\label{lemma g-5}
\end{lemma}
%%%%%%%%
Consider observables $\pi_{\tt{T}} = \alpha_{t_1},\alpha_{t_2} \dots \alpha_{t_n}$. 
We write $\pi_{\tt{T}} \lessapprox \pi'_{\tt{T}}$ to represent that $\pi'_{\tt{T}} = \pi_{\tt{T^0}} \cdot \alpha_{t_1} \cdot \pi_{\tt{T^1}} 
\cdot \alpha_{t_2} \cdot \pi_{\tt{T^2}} \dots \alpha_{t_n} \cdot \pi_{\tt{T^n}}$. 
In other words, $\pi_{\tt{T}}$ occurs as a non-contiguous subsequence in $\pi'_{\tt{T}}$. For such a $\pi_{\tt{T}}, \pi'_{\tt{T}}$, 
we define $\pi'_{\tt{T}} \oslash \pi_{\tt{T}} := \pi_{\tt{T^0}} \cdot \pi_{\tt{T^1}} \dots \pi_{\tt{T^n}}$. 
Since elements of $\pi_{\tt{T}}$ and $\pi'_{\tt{T}}$ are distinct, operation $\oslash$ is well defined. 
Let $\pi_{\tt{T}}[i]$ denote the $i$th observable 
in the observation sequence $\pi_{\tt{T}}$, and 
let  $|\pi_{\tt{T}}|$ denote  the number of observables 
in $\pi_{\tt{T}}$.

Let $\alpha_t = \pi_{\tt{T}}[i]$ for some $i: 1 \le i \le |\pi_{\tt{T}}|$. 
We define $\tt{Pre(\pi_{\tt{T}},\alpha_t)}$ as a subsequence $\pi'_{\tt{T}}$ of $\pi_{\tt{T}}$ such that  
(i) $\alpha_t \in \pi'_{\tt{T}}$,
(ii) $\alpha_{t_j} = \pi_{\tt{T}}[j] \in \pi'_{\tt{T}}$ for some $j: 1 \le j < i$ iff there exists $k: j < k \le i$ such that $\alpha_{t_k}=\pi_{\tt{T}}[k]  \in \pi'_{\tt{T}}$ and $\neg(\alpha_{t_j} \sim \alpha_{t_k})$. 
Thus, $\tt{Pre(\pi_{\tt{T}},\alpha_t)}$ consists of $\alpha_t$ and all 
$\alpha_{t'}$ appearing before $\alpha_t$ in $\pi_{\tt{T}}$ such that 
$t' [\tpo \cup \trf]^+ t$.

%
%
%%%%%%%
\begin{lemma}
If $\pi_{\tt{T^1}} = \tt{Pre(\pi_{\tt{T}},\alpha_t)}$ and $\pi_{\tt{T^2}} = \pi_{\tt{T}} \oslash \pi_{\tt{T^1}}$ then $\pi_{\tt{T}} \approx \pi_{\tt{T^1}} \cdot \pi_{\tt{T^2}}$.
\label{lemma g-6}
\end{lemma}
\begin{proof}
The proof is trivial since we can always execute in order, 
the $[\tpo \cup \trf]^+$ predecessors of $\alpha_t$ from $\tt{Pre(\pi_{\tt{T}},\alpha_t)}$, then $\alpha_t$, then the  observables 
in $\tt{Pre(\pi_{\tt{T}},\alpha_t)}$ which are independent from $\alpha_t$, followed by the suffix of $\pi_{\tt{T}}$ after $\alpha_t$.

\end{proof}

%%%%%%%
\begin{lemma}
If $\pi_{\tt{T}}= \pi'_{\tt{T}} \cdot \pi''_T$ and $\alpha_t \in \pi'_{\tt{T}}$ then $\tt{Pre(\pi_{\tt{T}},\alpha_t)} = \tt{Pre(\pi'_{\tt{T}},\alpha_t)}$.
\label{lemma g-7}
\end{lemma}
\begin{proof}
The proof is trivial once again, since 	all 
the transactions which are $[\tpo \cup \trf]^+ t$  are in the prefix  $\pi'_{\tt{T}}$.
\end{proof}

%%%%%%
\begin{lemma}
If $\langle \sigma,\tau \rangle \vdash_{\tt{G}} \pi_{\tt{T}}$ then $\langle \sigma,\tau \rangle \vdash_{\tt{G_T}} \pi_{\tt{T}} \cdot \pi_{\tt{T^2}}$.
\label{lemma g-8}
\end{lemma}
\begin{proof}
This simply follows from the fact that we can extend the observation sequence 
$\pi_{\tt{T}}$ to obtain a terminal configuration, since the DPOR algorithm generates weak traces corresponding to terminating runs.   	
\end{proof}

%%%%%%
\begin{lemma}
Consider a fulfilled trace $\tau$ such that $\tau \models \ccvt$, $\tau \vdash_{\tt{G}} \pi_{\tt{T}} \cdot \alpha_t$. Let each read event $ev_i = r_i(p,t,x_i,v)$ in $\alpha_t$ read from some transaction $t_i$, and let $\pi_{\tt{T}}$ be $t$-free.  Then $\tau \vdash_{\tt{G}} \alpha'_t \cdot \pi_{\tt{T}}$, where $\alpha'_t$ is the same as  $\alpha_t$, with the exception that the sources of its read events can be different. That is, 
 each read event $ev_i = r_i(p,t,x_i,v) \in \alpha'_t$ can read from some transaction $t'_i \neq t_i$.
\label{lemma g-9}
\end{lemma}
\begin{proof}
Let $\pi_{\tt{T}} = \alpha_{t_1} \alpha_{t_2} \dots \alpha_{t_n}$ and $\tau_0 \xrightarrow[]{\alpha_{t_1}}_{\sat} \tau_1 \xrightarrow[]{\alpha_{t_2}}_{\sat} \dots \xrightarrow[]{\alpha_{t_n}}_{\sat} \tau_n \xrightarrow[]{\alpha_t}_{\sat} \tau_{n+1}$, where $\tau_0 = \tau$. Let $\tau_i = \langle \tran_i, \tpo_i, \trf_i, \tco_i \rangle$. 
Let there be  $m$ read events in transaction $t$. Keeping in mind what we want to prove, where we want to execute $t$ first followed by $\pi_{\tt{T}}$, and obtain an execution $\alpha'_t \pi_{\tt{T}}$, we do the following.

For each read event $ev_i = r_i(p,t,x_i,v)$ we define $t'_i \in \tran^{w,x_i}$ such that 
$(i)$ $ t'_i \in \rbl(\tau_0,t,x_i)$, and 
$(ii)$ there is no $t''_i \in \rbl(\tau_0,t,x_i)$ where $t'_i [\tpo_n \cup \trf_n \cup \tco_n] t''_i$.  Note that this is possible since 
 $\pi_{\tt{T}}$ is $t$-free, so all the observables $\alpha_{t_i}$ occurring in $\pi_{\tt{T}}$ are such that $t_i$ is issued in a process other than that of $t$. Thus, when $\alpha_t$ is enabled, we can choose any of the 
 writes done earlier,  this fact is consistent with the $\ccvt$ semantics, since from Lemmas \ref{lem:f1}-\ref{lem:f4} we know $\tau_n \models \ccvt$.
Since $\tau_n \models \ccvt$ such a $t'_i \in  \rbl(\tau_0,t,x_i)$ exists for each $ev_i$.

\medskip 
Next we define a sequence of traces which can give the execution 
$\alpha'_t \pi_{\tt{T}}$. 
Define a sequence of traces $\tau'_0, \tau'_1, \dots \tau'_n$ where $\tau'_j = \langle \tran'_j, \tpo'_j, \trf'_j, \tco'_j \rangle$ is such that 
\begin{enumerate}
	\item $\tau \vdash_{\tt{G}} {\alpha'_t}$ and $\alpha'_t(\tau)=\tau'_0$,
	\item $\tau'_j \vdash_{\tt{G}} \alpha_{t_{j+1}}$ and  $\tau'_{j+1} = \alpha_{t_{j+1}}(\tau'_j)$ for all $j: 0 \le j \le n$.
\end{enumerate}

\begin{itemize}
\item  Define $\tran'_i = \tran_i \cup \{t\}$ for all $0 \leq i \leq n$, 
\item 
Define $\tpo' = \{t' [\tpo] t \mid t'$ is a transaction in $\tau$, in the same process as $t\}$, and $\tpo'_i = \tpo_i \cup \tpo'$ for all $0 \leq i \leq n$, 

\item  $\trf' = \bigcup_{i:1\le i \le m} t'_i [\trf^{x_i}] t$ (reads from relation corresponding to each read event $ev_i \in \alpha'_t$), and 
 $\trf'_i = \trf_i \cup \trf'$ for all $i : 1 \le i \le n$, 
 
\item  $\tco' = \bigcup_{j:1\le j \le m} \tco'_j$ (each  $\tco'_j$ corresponds to the updated $\tco$ relation because of the read transition $\xrightarrow[]{(read,t,t'_j)}_{\sat}$). 	
\smallskip 

For $1 \leq i \leq n$, we define $\tco'_i$ inductively as $\tco'_i = \tco_i \cup \tco'$ and show that $\tau'_i \vdash_{\tt{G}} \alpha_{t_{i+1}}$ and  $\tau'_{i+1} = \alpha_{t_{i+1}}(\tau'_i)$ holds good. 
 First define $\tco'_0 = \tco_0 \cup \tco'$. Then define  $\tco'_i$ to be the coherence order corresponding to $\alpha_{t_{i}}(\tau'_{i-1})$  where $\tau'_{i-1}=\langle \tran'_{{i-1}}, \tpo_{i-1}, \trf_{i-1}, \tco_{i-1} \rangle$ for all $i: 1 \le i \le n$. 

 \end{itemize}

\medskip 
\noindent{\bf{Base case}}. The base case $\tau \vdash_{\tt{G}} {\alpha'_t}$ and $\alpha'_t(\tau)=\tau'_0$,
   holds trivially, by construction. 

\smallskip 

\noindent{\bf{Inductive hypothesis}}. Assume that $\tau'_j \vdash_{\tt{G}} \alpha_{t_{j+1}}$ and  $\tau'_{j+1} = \alpha_{t_{j+1}}(\tau'_j)$ for $0 \leq j \leq i-1$. 

\smallskip 

 We have to prove that 
$\tau'_i \vdash_{\tt{G}} \alpha_{t_{i+1}}$ and  $\tau'_{i+1} = \alpha_{t_{i+1}}(\tau'_i)$. 
\begin{enumerate}
	\item If $t_{i+1} \in \tran^{w}$ and $t_{i+1} \notin \tran^r$,  then the proof holds trivially from the inductive hypothesis. 
	\item Consider now $t_{i+1} \in \tran^r$. Consider a read event 
	$ev^{i+1} = r(p,t_{i+1},x,v) \in \alpha_{t_{i+1}}$ which was reading from 
	transaction $t_x$ in $\pi_{\tt{T}}$. That is, we had $t_x \in \rbl(\tau_i, t_{i+1},x)$. 	If $t_x \in \rbl(\tau'_i, t_{i+1},x)$, then we are done, since we can simply extend the run from the inductive hypothesis. 
	
	\smallskip 
	
	Assume otherwise. That is, $t_x \notin \rbl(\tau'_i, t_{i+1},x)$.

	Since  $t_x$  $\in$   $\rbl(\tau_i, t_{i+1},x)$, we know that there are some blocking transactions in the new path which prevents $t_x$ from being readable. Basically, we have the blocking transactions since $t$ is moved before $\pi_{\tt{T}}$. 	
	
	\begin{itemize}
		\item Consider $tr_1 \in \vbl(\tau,t,y)$ for some variable $y$ such that,  in $\pi_{\tt{T}}.\alpha_t$, we had $t_x [\tpo_i \cup \trf_i \cup \tco_i]^* tr_1$. This path
		 is possible since $\alpha_t$ comes last in in $\pi_{\tt{T}}.\alpha_t$,  after  $\alpha_{t_{i+1}}$. 
		\item  Consider $tr_2 \in \vbl(\tau_i,t_{i+1},x)$.  Since $t_x$ $\in$ $\rbl(\tau_i, t_{i+1},x)$, we have  $tr_2 [\tco^x_{i+1}] t_x$. 
Now, in $\alpha'_t.\pi_{\tt{T}}$, assume $tr_3 [\trf'^y_0] t$, 
such that we have a path from $tr_3$ to $t_x$, as  $tr_3 [\tpo_i \cup \trf_i \cup \tco_i]^* tr_2$. 
	\end{itemize}
	  		  Hence it follows that $tr_3 [\tpo_i \cup \trf_i \cup \tco_i]^* tr_2$ 
$[\tco^x_{i+1}] t_x$ $[\tpo_i \cup \trf_i \cup \tco_i]^* tr_1$. 
Hence we have $tr_3 [\tpo_{i+1} \cup \trf_{i+1} \cup \tco_{i+1}]^+ tr_1$, i.e 
$tr_3 [\tpo_n \cup \trf_n \cup \tco_n]^+ tr_1$. This leads to the contradiction since $tr_1 \in \vbl(\tau,t,y)$ and  $tr_3 [\trf'^y_0] t$.  

Hence, $t_x$  $\in$   $\rbl(\tau_i, t_{i+1},x)$ and we can extend the run 
from the inductive hypothesis obtaining $\tau'_j \vdash_{\tt{G}} \alpha_{t_{j+1}}$,  $\tau'_{j+1} = \alpha_{t_{j+1}}(\tau'_j)$,  
for $0 \leq j \leq i-1$,
and 
$\tau'_i \vdash_{\tt{G}} \alpha_{t_{i+1}}$. 

%%%t'_3=t_1
%%%t'_4=t_2, 
%%%%t'_5=_3

%	
%		
%	Assume that $t'_i \notin \rbl(\tau'_i , t_{i+1},x)$ such that some read event $ev^{i+1} = r(p_{i+1}, t_{i+1},x,v) \in \alpha_{t_{i+1}}$ reads from $t'_{i+1}$ in $\tau_{i+1}$, i.e $t'_{i+1} \in \rbl(\tau_i,t_{i+1},x)$. We show that this leads to contradiction.

\end{enumerate}

%Since $t'_i \notin \rbl(\tau'_i , t_{i+1} , x)$ and $t'_i \in \rbl(\tau_i , t_{i+1},x)$ 
%we know that there are transactions $t'_3 \in \vbl(\tau_0,t,y)$ and  
%$\tau_4 \in \vbl(\tau_i,t_{i+1},x)$ such that $t'_5 [\trf'^y_0] t$ , $t'_i [\tpo_i \cup \trf_i \cup \tco_i]^* t'_3$, $t'_5 [\tpo_i \cup \trf_i \cup \tco_i]^* t'_4$.
Now we prove that $\tco'_{i+1} = \tco_{i+1} \cup \tco'$. 
Assume we have $(tr1 , tr2) \in \tco_{i+1}$. We show that $(tr1 , tr2) \in \tco'_{i+1}$. We have the following cases:

\begin{itemize}
    \item[(i)] $(tr1 , tr2) \in \tco_i$. From the inductive hypothesis it follows that $(tr1 , tr2) \in \tco'_{i}$ and hence in $\tco'_{i+1}$.
    \item[(ii)] $(tr1 , tr2) \notin \tco_i$ and some read event $ev = r(p,t_{i+1},x,v)$ from $\alpha_{t_{i+1}}$ reads from $tr2$.  That is, $tr1,tr2 \in \rbl(\tau_i, t_{i+1},x)$ and $tr1 \in \vbl(\tau_i,t_{i+1},x)$.
    Assume $(tr1 , tr2) \notin \tco'_{i+1}$.
    Since $(tr1, tr2) \notin \tco'_{i+1}$, it follows that there exists  $tr3 \in \vbl(\tau'_i,t_{i+1},x)$ such that $tr2 [\tpo'_i \cup \trf'_i \cup \tco'_i] tr3$. This means $tr2 \in \rbl(\tau_i,t_{i+1},x)$, but 
    $tr2 \notin \rbl(\tau'_i,t_{i+1},x)$. However,  as proved earlier, this leads to a contradiction. 

\end{itemize}
Thus, we have shown that $\tau \vdash_{\tt{G}} \alpha'_t \alpha_{t_1} \dots \alpha_{t_i}$ 
is such that $\alpha'_t \alpha_{t_1} \dots \alpha_{t_i}(\tau)=\tau'_i$ for all 
$0 \leq i \leq n$. When $i=n$ we obtain 
$\alpha'_t \pi_{\tt{T}}(\tau)=\tau'_n$, or $\tau \vdash_{\tt{G}} \alpha'_t \pi_{\tt{T}}$. 
%\qed 
\end{proof}

%%%%%%%%

\begin{definition}[Linearization of  a Trace]
A observation sequence $\pi_{\tt{T}}$ is a \emph{linearization} of a trace $\tau = \langle \tran, \tpo , \trf, \tco \rangle$ if $(i)$ $\pi_{\tt{T}}$ has the same transactions as $\tau$ and $(ii)$ $\pi_{\tt{T}}$ follows the ($\tpo \cup \trf)$ relation.
	
\end{definition}

We say that our DPOR algorithm \emph{generates an observation sequence} $\pi_{\tt{T}}$ from state $\langle \sigma, \tau \rangle$ where $\sigma$ is a configuration and $\tau$ is a trace if 
 it invokes $ExploreTraces$ with parameters $\sigma,\tau, \pi'$, where $\pi'$ is a \emph{linearization} of $\tau$, and generates  a sequence of recursive calls to $ExploreTraces$ resulting in $\pi_{\tt{T}}$.

\begin{lemma}
If $\langle \sigma,\tau \rangle \vdash_{\tt{G_T}} \pi_{\tt{T}}$ then, 
the DPOR algorithm  generates $\pi'_{\tt{T}}$ from state $\langle \sigma,\tau \rangle$ 
for some $\pi'_{\tt{T}} \approx \pi_{\tt{T}}$.
\label{lemma g-10}
\end{lemma}
\begin{proof}
We use induction on $|\pi_{\tt{T}}|$. If $\sigma$ is $terminal$, then the  proof is trivial.
Assume that we have $\langle \sigma,\tau \rangle \vdash_{\tt{G_T}} \pi_{\tt{T}}$.
Assume that $\langle \sigma,\tau \rangle \vdash_{\tt{G}} \alpha_t$. It follows that $\langle \sigma,\tau \rangle \vdash_{\tt{G}} \alpha_t$.
Using Lemma \ref{lemma g-5} we get $\pi_{\tt{T}} = \pi_{\tt{T^1}} \cdot \alpha_t \cdot \pi_{\tt{T^2}}$, where $\pi_{\tt{T^1}}$ is $t$-free. 
We consider the following two cases:
\begin{itemize}
    \item In the first case, we assume that all read events in $t$ read from 
    transactions in $\tau$. So in this case, $\pi_{\tt{T^1}}$ can be empty. 
        Assume there are $n$ read events in $t$ and each read event $ev_i = r(p,t,x_i,v)$ 
    reads from transactions $t_i \in \tau$ for all $i: 1 \le i \le n$. 
In this case the DPOR algorithm will let each read event $ev_i$ read from all possible transactions $t' \in \rbl(\tau,t,x_i)$, including $t_i$.
    \item In the second case, assume that there exists at least one read event $ev' = r(p,t,x,v) \in \alpha_t$ which reads from a transaction $t' \in \pi_{\tt{T^1}}$ (hence, $\pi_{\tt{T^1}}$ is non empty).
    \smallskip 
     
    %Let $\pi_{\tt{T^3}} = \tt{Pre(\pi_{\tt{T^1}}, \alpha_t)}$.
    From Lemma \ref{lemma g-9}, we know that $\langle \sigma,\tau \rangle
    \vdash_{\tt{G}} \alpha'_t \cdot \pi_{\tt{T^1}}$. 
    From Lemma \ref{lemma g-8}, it follows that $\langle \sigma,\tau \rangle
    \vdash_{\tt{G_T}} \alpha'_t \cdot \pi_{\tt{T^1}} \cdot \pi_{\tt{T^4}}$, for some
    $\pi_{\tt{T^4}}$.
    Hence there exists $\langle \sigma',\tau' \rangle$ such that 
    $\langle \sigma',\tau' \rangle = \alpha'_t (\langle \sigma,\tau
    \rangle)$ and $\langle \sigma',\tau' \rangle \vdash_{\tt{G_T}} \pi_{\tt{T^1}} \cdot
    \pi_{\tt{T^4}}$. 
    
    Since $|\pi_{\tt{T^1}} \cdot
    \pi_{\tt{T^4}}| < |\pi_{\tt{T}}$, we can use the inductive hypothesis. It follows that the DPOR algorithm generates from state $\langle \sigma',\tau' \rangle$, 
    the observation sequence  $\pi_{\tt{T^5}}$ such that $\pi_{\tt{T^5}} \approx \pi_{\tt{T^1}} 
    \cdot \pi_{\tt{T^4}}$. 
    
    \smallskip 
    
    Let  $\pi_{\tt{T^3}}.\alpha_t = \tt{Pre(\pi_{\tt{T^1}}, \alpha_t)}$. Then  $\pi_{\tt{T^5}}
    \approx \pi_{\tt{T^1}} \cdot \pi_{\tt{T^4}}$ implies that  $\pi_{\tt{T^3}}
    \lessapprox \pi_{\tt{T^5}}$ (by applying Lemma \ref{lemma g-7}).
%    Since $\pi_{\tt{T^3}}$ is $t$-free it follows that $\langle \sigma,\tau     \rangle \vdash_{\tt{G}} \pi_{\tt{T^3}} \cdot \alpha_t$. 
    Let $\pi_{\tt{T^6}} \approx \pi_{\tt{T}} \oslash (\pi_{\tt{T^3}} \cdot \alpha_t)$.
    By applying Lemma \ref{lemma g-6}, we get $\pi_{\tt{T}} \approx \pi_{\tt{T^3}} \cdot \alpha_t \cdot \pi_{\tt{T^6}}$.
    Since $\langle \sigma,\tau \rangle \vdash_{\tt{G_T}} \pi_{\tt{T}}$ and 
    $\pi_{\tt{T}} \approx \pi_{\tt{T^3}} \cdot \alpha_t \cdot \pi_{\tt{T^6}}$,
    by applying Lemma \ref{lemma g-3}, we get $\langle \sigma,\tau \rangle
    \vdash_{\tt{G_T}} \pi_{\tt{T^3}} \cdot \alpha_t \cdot \pi_{\tt{T^6}}$.
    Let $\langle \sigma',\tau' \rangle = (\pi_{\tt{T^3}} \cdot \alpha_t) (\langle \sigma,\tau \rangle)$. 
    Since $\langle \sigma,\tau \rangle \vdash_{\tt{G_T}} \pi_{\tt{T^3}} 
    \cdot \alpha_t \cdot \pi_{\tt{T^6}}$, we have $\langle \sigma',\tau' \rangle
    \vdash_{\tt{G_T}} \pi_{\tt{T^6}}$. 
    From inductive hypothesis it follows that $\langle \sigma',\tau' \rangle$ generates $\pi_{\tt{T^7}}$ such that $\pi_{\tt{T^7}} \approx \pi_{\tt{T^6}}$.\\
    In other words, $\langle \sigma,\tau \rangle$ generates $\pi_{\tt{T^3}} 
    \cdot \alpha_t \cdot \pi_{\tt{T^7}}$ where $\pi_{\tt{T}} \approx \pi_{\tt{T^3}} 
    \cdot \alpha_t \cdot \pi_{\tt{T^7}}$.
\end{itemize}

\end{proof}

\newpage 
